# Supplementary material for: Light-sheet microscopy with attenuation-compensated propagation-invariant beams
Source: arXiv:1708.02612 ancillary file (2017-08-17)
Supplement: Supplementary file 1 [file SupplementaryInformation.pdf]

# Light-sheet microscopy with attenuation-compensated propagation-invariant beams

Jonathan Nylk[1,*], Kaley McCluskey[1,†], Miguel A. Preciado[1,‡], Michael Mazilu[1], Frank J. Gunn-Moore[2], Sanya Aggarwal[3], Javier A. Tello[3], David E. K. Ferrier[4], and Kishan Dholakia[1]

[1]SUPA, School of Physics and Astronomy, University of St Andrews, North Haugh, St Andrews, KY16 9SS

[2]School of Biology, University of St Andrews, North Haugh, St Andrews, KY16 9SS

[3]School of Medicine, University of St Andrews, North Haugh, St Andrews, KY16 9SS

[4]Scottish Oceans Institute, Gatty Marine Laboratory, School of Biology, University of St Andrews, East Sands, St Andrews, KY16 8LB

## Supplementary Materials


| Note # | Title | Page # |
|---|---|---|
| S1 | Attenuation-compensation of an Airy beam light-sheet | S1 |
| S2 | Attenuation-compensation of a Bessel beam light-sheet | S5 |
| S3 | Modification of deconvolution protocol incorporating attenuation and attenuation-compensation | S9 |
| S4 | Theoretical imaging performance of attenuation-compensated Airy beam light-sheet | S11 |
| S5 | Effect of incorrect attenuation estimation on deconvolution | S13 |
| S6 | Theoretical imaging performance of attenuation-compensated Bessel beam light-sheet | S15 |
| S7 | Determination of specimen attenuation | S18 |
| S8 | Sample-based geometric effects on attenuation | S19 |
| S9 | Attenuation-compensation of multi-photon excitation Airy and Bessel light-sheets | S20 |
| S10 | Additional Supplementary Figures and Tables | S24 |


*email: jn78@st-andrews.ac.uk

†Present address: Department of Bionanoscience, Kavli Institute of Nanoscience, Delft University of Technology, Van der Maasweg 9 2629HZ Delft, The Netherlands

‡Present address: School of Physics and Astronomy, University of Glasgow, Glasgow, G12 8QQ, UK

# S1 Attenuation-compensation of an Airy beam light-sheet

The following Note summarises the approach to attenuation compensation of Airy beams as described by Preciado, Dholakia, and Mazilu [30]. This approach is expanded and discussed in the context of light-sheet microscopy. Throughout this discussion, we are consistent with the microscope coordinate system we have defined earlier, with the illumination propagation along the $x-$axis and optic axis of the detection optics along the $z-$axis.

### Derivation of attenuation-compensation Airy field equation in linearly attenuating medium

The spatial Fourier spectrum of a 1+1D (1 lateral dimension + 1 longitudinal dimension) Airy beam propagating through a linearly absorbing medium can be approximated as:

$$\tilde{E}(k_z, x) \approx \exp\left(\frac{ik_z^2 x}{2nk_0 - iC_{abs}} - ink_0 x - \frac{C_{abs}x}{2}\right)\exp\left(\frac{iz_0^3 k_z^3}{3}\right) \tag{S1}$$

where $k_z$ is the spatial frequency of the transverse coordinate, $z$, $x$ is the longitudinal coordinate, $k_0 = 2\pi/\lambda$ is the vacuum wave vector, $z_0$ is a scaling factor that dictates the extent of the Airy beam, and $n$ and $C_{abs}$ are the refractive index and absorption coefficient of the absorbing medium respectively.

The Fourier transform of (S1) yields the propagation of the Airy field in the absorbing medium:

$$E(z, x) = \text{Ai}\left(\frac{z}{z_0} - \frac{x^2}{4x_0^2}\right)\exp\left(-\frac{C_{abs}x}{2}\right)\exp\left(i\left[\frac{x^3}{12x_0^3} - \frac{x_0 x}{z_0^2} - \frac{zx}{2z_0 x_0}\right]\right) \tag{S2}$$

where $x_0 = nk_0 z_0^2$.

The middle term, $\exp(-C_{abs}x/2)$, characterises the decay of the field upon propagation. As this stems from a real exponential term in the Fourier spectrum of the beam, it can be accounted for by introducing another exponential, $\exp(-b_0 k_z)$ which results in the field equation:

$$\begin{aligned} E(z, x) = \text{Ai}\left(\frac{z}{z_0} - \frac{x^2}{4x_0^2} + \frac{ib_0}{z_0}\right)\exp\left(-\frac{C_{abs}x}{2} + \frac{xb_0}{2z_0 x_0}\right) \\ \exp\left(i\left[\frac{x^3}{12x_0^3} - \frac{x_0 z}{z_0^2} - \frac{zx}{2z_0 x_0}\right]\right) \end{aligned} \tag{S3}$$

The total intensity loss due to absorption, $C'_{abs}$, is now given by:

$$C'_{abs} = C_{abs} - \frac{b_0}{z_0 x_0} \tag{S4}$$

For $b_0 = z_0 x_0 C_{abs}$, the beam will completely counteract attenuation and the intensity of the main lobe will propagate without decay, as if in free-space. In free-space, $b_0 \neq 0$ will result in a beam where the intensity of the main lobe increases or decreases with propagation.

For a light-sheet with a cylindrical pupil function $P \equiv P(k_z)$ the above expressions are sufficient but this treatment can easily be extended to 2+1D Airy beams ($P \equiv P(k_z, k_y)$), where the overall compensation is the sum of the compensation along each individual axis:

$$C'_{abs} = C_{abs} - \frac{b_{0z}}{z_0 x_0} - \frac{b_{0y}}{y_0 x_0} \tag{S5}$$

Attenuation-compensation is essentially the application of an amplitude mask in the pupil plane which weights each spectral component based on the path length of that component before it contributes to the main lobe of the beam. The above treatment considers only attenuation in a linearly absorbing medium ($C_{abs} = constant$), but it can be readily applied to complex systems where non-linear attenuation is encountered ($C_{abs} \equiv C_{abs}(x)$).

### Ray optics approach to attenuation-compensation of Airy beam

Attenuation-compensation can be considered from a ray optics perspective as is shown in Fig. S1. The ray optics representation readily shows how the characteristic parabolic shape of the main caustic of the Airy beam arises from the cubic phase profile in the pupil plane. In an attenuating

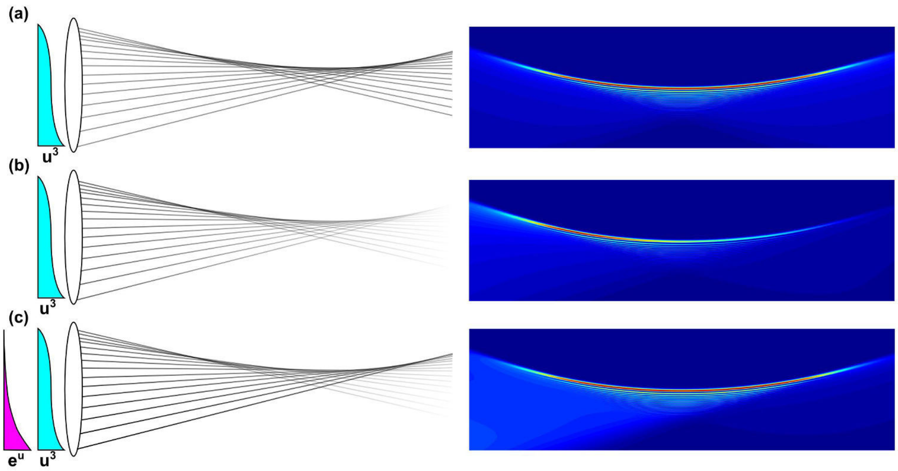


Figure S1: Ray optics representation of an Airy beam (left) and wave optics simulations (right). (a) Airy beam in free-space formed by a cubic ($\propto u^3$) phase term. (b) Airy beam in linearly attenuating medium. (c) Airy beam in linearly attenuating medium with attenuation-compensation performed by exponentially increasing the amplitude of the rays that form the main caustic of the Airy beam at greater distances from the lens ($\propto \exp(u)$).

medium, all the rays attenuate at equal rates but the rays which form the caustic furthest from the lens have travelled further than rays that form earlier parts of the caustic and have also therefore attenuated more at this point. Attenuation-compensation is achieved when the amplitude of each ray, at the point it forms the main caustic, is equal.

**Normalised pupil function for an attenuation-compensated Airy light-sheet**

The cylindrical pupil function of an attenuation-compensated Airy light-sheet is given by:

$$P(u) = A_\sigma \exp(2\pi i \alpha u^3) \exp(-u^8) \exp(\sigma[u-1]) H(\sqrt{2} - |u|) \tag{S6}$$

where $u$ in the normalised pupil coordinate corresponding to the $z-$axis, $A_\sigma$ is a real scaling factor, $\alpha$ dictates the propagation-invariance of the Airy light-sheet [11], $\sigma$ dictates the degree of linear attenuation-compensation, and $H(\cdot)$ denotes the Heaviside step function. The addition of the "soft-edge" 8th-order super-Gaussian apodization function (middle term in eq. (S6)) is used to eliminate sharp discontinuities which occur at the edge of the pupil function when attenuation-compensation is used and is consistent with the approach of Preciado, Dholakia, and Mazilu [30]. To accommodate the "soft-edge" of this pupil function, the "hard-edge" apodization ($H(\cdot)$) is extended from $|u| = 1$ to $|u| = \sqrt{2}$. $A_\sigma$ is chosen such that the maximum amplitude of the pupil function with any $\sigma$ is unity and such that all light-sheets have the same peak intensity at the beginning of their field-of-view (FOV).

Experimentally, our light-sheet is formed either by cylindrical focussing of a 1+1D Airy beam with pupil function given by (S6) or by digital scanning of a spherically focussed 2+1D Airy beam [11] with pupil function given by:

$$\begin{aligned} P(u,v) =& A_\sigma \exp(2\pi i \alpha[u^3 + v^3]) \exp(-u^8) \exp(\sigma_u[u-1]) \\ & \exp(-v^8) \exp(\sigma_v[v-1]) H(\sqrt{2} - \sqrt{u^2+v^2}) \end{aligned} \tag{S7}$$

where the pupil function remains separable in Cartesian coordinates ($P(u,v) = P(u)P(v)$, except for minor contributions from $H(\cdot)$), and $\sigma_u$ and $\sigma_v$ denote modulation along the $u-$ and $v-$axes respectively.

Due to the separable nature of (S7) and the fact that the focussed beam is scanned along the $y - axis$ for formation of the light-sheet, the exact form of $P(v)$ is somewhat irrelevant to the cross-section of the light-sheet as long as the scan range is larger than the $y-$axis transverse extent of the beam. We therefore set $\sigma_v = 0$ in all further discussions and (S6) is an accurate description of the light-sheet pupil function. Modulation only compensates for attenuation of the light-sheet

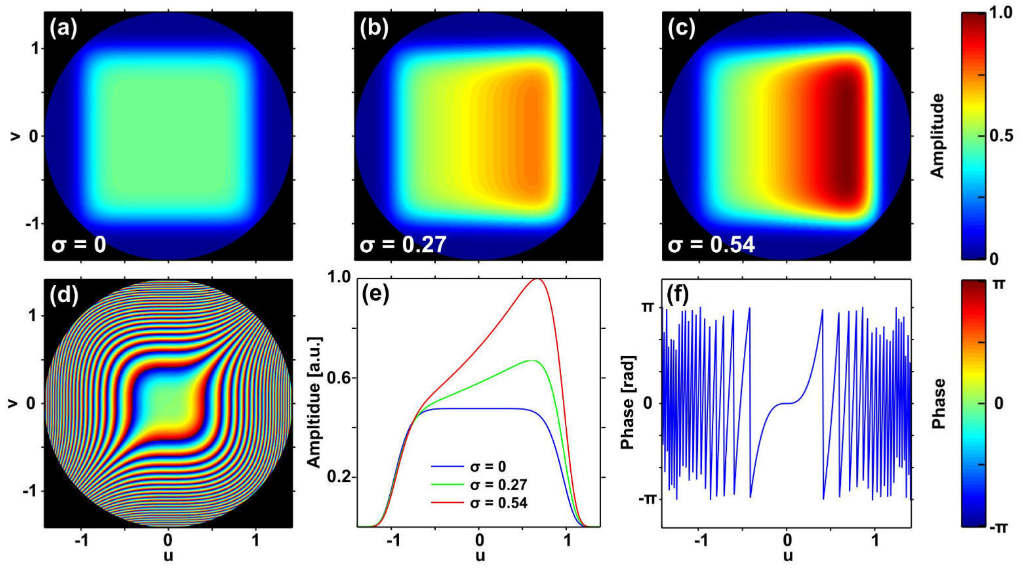


Figure S2: Spherical attenuation-compensated Airy beam amplitude (a-c) and phase (d) pupil functions and their cylindrical (e,f) counterparts respectively. For all $\sigma$, the phase profile (d,f) is unaffected.

profile when applied along the $u-$axis. Figure S2 shows examples of the pupil functions given by (S6) and (S7).

**Attenuation-compensated Airy light-sheet in terms of normalised pupil parameters**

Considering the normalised pupil functions used to describe an Airy light-sheet, the transverse coordinate, $k_z$ is related to the normalised transverse coordinate, $u$, by:

$$u = k_z \frac{\lambda}{2\text{NA}} \tag{S8}$$

Similarly, $z_0$ and $\alpha$, and $b_0$ and $\sigma$ are related by the following equations:

$$\alpha = \frac{1}{6\pi}\left(\frac{2\text{NA}z_0}{\lambda}\right)^3 \tag{S9}$$

$$\sigma = b_0 \frac{2\text{NA}}{\lambda} \tag{S10}$$

We denote the second term of (S4) $\chi$, the degree of compensation. Re-expressed in terms of normalised coordinates this becomes:

$$\chi = \frac{\sigma \text{NA}^2}{3\pi^2 n\alpha\lambda} \tag{S11}$$

We find (S11), derived from [30], to be a factor of 10 underestimated compared to simulations and experimental evidence and therefore include this factor as an empirical constant in $\chi$:

$$\chi = \frac{10\sigma \text{NA}^2}{3\pi^2 n\alpha\lambda} \tag{S12}$$

This empirical constant is implicitly included in all references to $\chi$ throughout the Main Text and Supplement of this manuscript. Any reference to $\chi$ refers to (S12).

There is little that limits the degree of compensation that can be achieved for an Airy beam with a given $\alpha-$parameter other than the amount of power that can be delivered in the beam. More practically for imaging, though, the extra energy delivered to deeper locations of the beam causes a non-negligible distortion of the beam profile (Fig. S1(c)). As the rays of the main caustic at greater depth influences the side-lobe structure earlier in propagation, the extra energy added to the beam causes the intensity of the side-lobes to increase. We define a practical limit for the

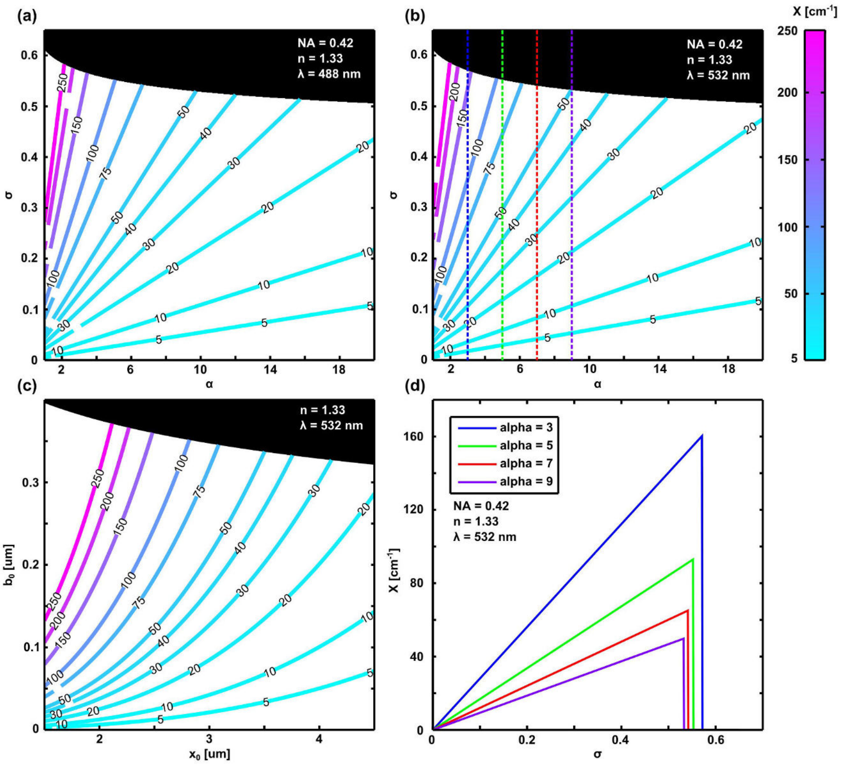


Figure S3: Look up tables for attenuation-compensated Airy light-sheet. Contour plot showing lines of constant $\chi$ for combinations of $\alpha-$ and $\sigma-$values for (a) $\lambda$ = 488 nm and (b) $\lambda$ = 532 nm. (c) Same plot as (b) but expressed in terms of real-space parameters, $x_0$ and $b_0$. (d) lines profiles taken through (b) for selected $\alpha-$values. Black regions in (a-c) indicate forbidden regions not satisfying the limits defined in (S14) and (S15).

maximum attenuation-compensation that can be applied as the degree of compensation at which the peak transverse intensity of the beam no longer follows the parabolic trajectory expected of the Airy beam within the longitudinal range set by the FOV of the Airy beam as given by:

$$FOV_{Airy} = \frac{6\alpha\lambda}{n}\frac{1}{1-\sqrt{1-(\mathrm{NA}/n)^2}} \tag{S13}$$

Using these criteria, and simulations of beam profiles with various $\alpha-$ and $\sigma-$parameters, compensation must satisfy the following inequality:

$$\alpha^{0.0635}\sigma \leq 0.6125 \tag{S14}$$

or expressed in real-space parameters:

$$x_0^{3\times 0.0635} b_0 \leq 0.6125(6\pi)^{0.0635}\left(\frac{\lambda}{2\mathrm{NA}}\right)^{(3\times 0.0635)+1} \tag{S15}$$

It is expected that different choices of "soft-edge" apodization in the pupil function will yield different results for the maximum permitted compensation, as well as small differences in the maximum achievable FOV.

Figure S3 shows the degree of compensation, $\chi$, that can be achieved for $\alpha-$values commonly used for light-sheet microscopy [11]. The lines of constant $\chi$ in Fig. S3(a,b) define a linear relation between $\sigma$ and $\alpha$. This is fundamentally linked to the relationship between the FOV and the $\alpha-$parameter of the Airy beam. If the FOV is doubled in a given linearly attenuating medium, the total attenuation across the FOV will also double, and so the $\sigma-$parameter will also have to be doubled to maintain full attenuation-compensation. The product of $\chi$, for a given $\sigma-$parameter, and the FOV is a constant.

## S2 Attenuation-compensation of a Bessel beam light-sheet

The following Note summarises the approach to attenuation-compensation of Bessel beams as described by Čižmár and Dholakia [27]. Throughout this discussion, we are consistent with the microscope coordinate system we have defined earlier, with the illumination propagation along the $x-$axis and optic axis of the detection optics along the $z-$axis.

### Derivation of method for producing Bessel beam with arbitrary axial envelope

The spatial Fourier transform of an azimuthally independent beam ($E(r, x = 0)$), such as a Bessel beam, can be expressed as a zero-order Hankel transform:

$$\tilde{E}(k_r, x = 0) = \int_0^\infty E(r, x = 0) J_0(k_r r) r dr \tag{S16}$$

where $k_r = \sqrt{k_z^2 + k_y^2}$ is the wave vector of $r = \sqrt{z^2 + y^2}$, $x$ is the longitudinal coordinate, and $J_0(k_r r)$ is the zero-order Bessel function.

It then follows by the inverse transform of (S16) that, for a Bessel beam, the on-axis propagation of the field ($E(r = 0, x)$) is linked with the radial mapping of the pupil ($\tilde{E}(k_r, x = 0)$) by:

$$E(r = 0, x) = \int_0^k \tilde{E}(k_r, x = 0) \exp(ik_x x) dk_x \tag{S17}$$

where $k_x = \sqrt{k_0^2 - k_r^2}$ and $k_0 = 2\pi/\lambda$ is the vacuum wave vector.

For a quasi-Bessel beam, $E_{Bessel}(r = 0, x) = A(x) \exp(ik_{x_0} x)$, where $A(x)$ is the desired axial envelope function, $k_{x_0} = \sqrt{k^2 - k_{r_0}^2}$, $k_{r_0}$ is the radial wave vector corresponding to an ideal Bessel spectrum, the radial pupil function that can yield this envelope is found by the transform:

$$\tilde{E}(k_r, x = 0) = \frac{1}{2\pi k_x} \int_{-\infty}^{\infty} A(x) \exp(ik_{x_0} x) \exp(-ik_x x) dx \tag{S18}$$

A quasi-Bessel beam with a uniform intensity profile can be generated using a pupil function determined by solving (S18) with the axial envelope defined by:

$$A_{uniform}(x) = \begin{cases} 1 & \text{if } |x| \leq x_{max} \\ 0 & \text{if } |x| > x_{max} \end{cases} \tag{S19}$$

where $2x_{max}$ is the maximum longitudinal extent of the Bessel beam.

To compensate for attenuation in a linearly absorbing medium, we have already established that the beam intensity must increase exponentially on propagation. Quasi-Bessel beams with exponentially increasing intensity on-axis can be generated from (S18) with the axial envelope defined by:

$$A_\sigma(x) = \begin{cases} \exp(\sigma x / x_{max}) & \text{if } |x| \leq x_{max} \\ 0 & \text{if } |x| > x_{max} \end{cases} \tag{S20}$$

where $\sigma$ is a constant that controls the degree of linear attenuation-compensation.

Consistent with the method described by Čižmár and Dholakia [27], and similarly to the method presented by Preciado, Dholakia, and Mazilu [30], a "soft-edge" apodization is applied to the determined pupil function in order to suppress high-frequency on-axis field oscillations which would otherwise distort the desired intensity profile. The apodization is a radial Gaussian centred on $k_{r_0}$ with a width of $k_{r_0}/4$:

$$\tilde{E}_{apodization}(k_r, x = 0) = \exp\left(\frac{-8(k_r - k_{r_0})^2}{k_{r_0}^2}\right) H\left(\sqrt{2} - k_r \frac{\lambda}{2\text{NA}}\right) \tag{S21}$$

where $H(\cdot)$ is the Heaviside step function which limits the pupil to a finite extent and is consistent with our approach in Supp. Note S1.

Figure S4 shows numerically determined radial pupil function profiles for attenuation-compensated Bessel beams with various degrees of compensation.

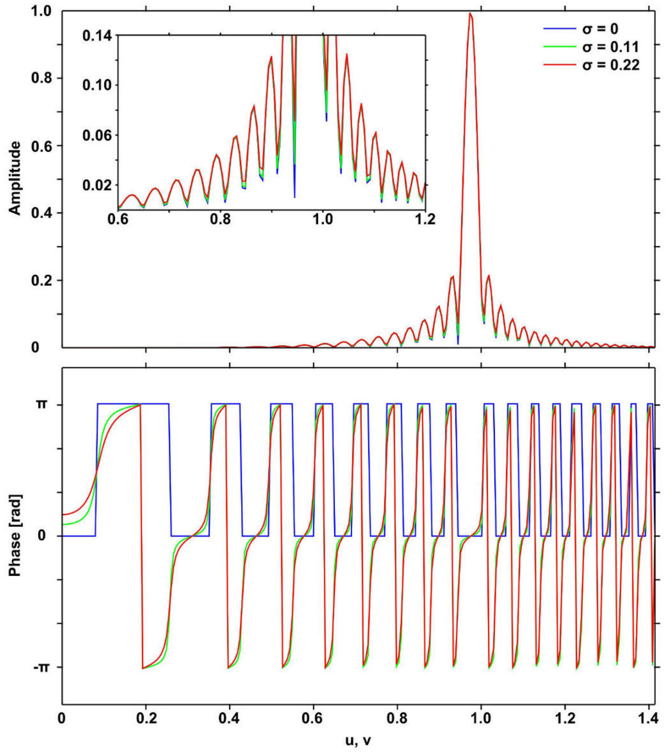


Figure S4: Amplitude (top) and phase (bottom) of radial pupil functions for attenuation-compensated Bessel beams with $\beta = 0.05$, $\lambda = 532$nm, NA $= 0.42$, and $n = 1.33$. Inset shows finer detail of amplitude structure. Blue: $\sigma = 0$ (no compensation, uniform on-axis profile); green: $\sigma = 0.11$; red: $\sigma = 0.22$ ($\chi = 65\text{cm}^{-1}$). Pupil amplitudes have been normalised to their maximum value for display.

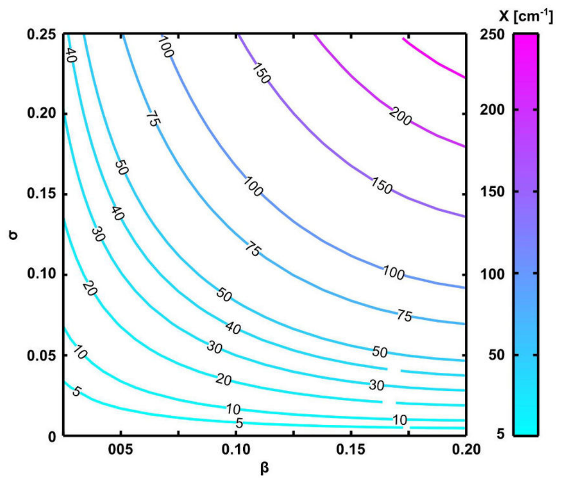


Figure S5: Look up table for compensated Bessel beam. Contour plot showing lines of constant $\chi$ for combinations of $\beta-$ and $\sigma-$values for $\lambda = 532$ nm, NA $= 0.42$, $n = 1.33$.

## Attenuation-compensation of a Bessel beam versus a Bessel light-sheet

Through numerical determination of the pupil function for attenuation-compensating Bessel beams and beam propagation simulations in linearly absorbing media, the relationship between compensation parameter, $\sigma$, and the degree of compensation, $\chi$, was determined and is shown in Fig. S5. The lines of constant $\chi$ define an inverse relationship ($\sigma \propto \beta^{-1}$). This is consistent with the trend between $\alpha$ and $\sigma$ observed in Fig. S3 as the FOV of a Bessel light-sheet scales inversely with $\beta$ [11].

As the Bessel beam is not separable in Cartesian coordinates, a Bessel light-sheet must be formed from a digitally scanned spherically focussed Bessel beam. As the attenuation-compensated Bessel beam is circularly symmetric, digital scanning along the $y-$axis reduces the efficacy of the compensation. This can be seen in Fig. S6 which shows an attenuation-compensated Bessel beam which yields no net attenuation ($C'_{abs} = 0$; Fig. S6(q-x)) and their corresponding light-sheet cross-sectional profiles.

The reduction in $\chi$ with digital scanning of a Bessel beam may not be as much of an issue for Bessel beam based light-sheet microscopy as first thought. It has already been shown that digitally scanned Bessel light-sheet microscopy gives poor optical sectioning in the single-photon excitation regime [11, 15] and successful implementations almost exclusively rely on stepped Bessel beams in tandem with a synchronised confocal line aperture [14, 24, 33, 34] or arrays of Bessel beams and structured illumination principles [16, 18] to achieve optical sectioning. Attenuation-compensation is compatible and complimentary with all of these methods.

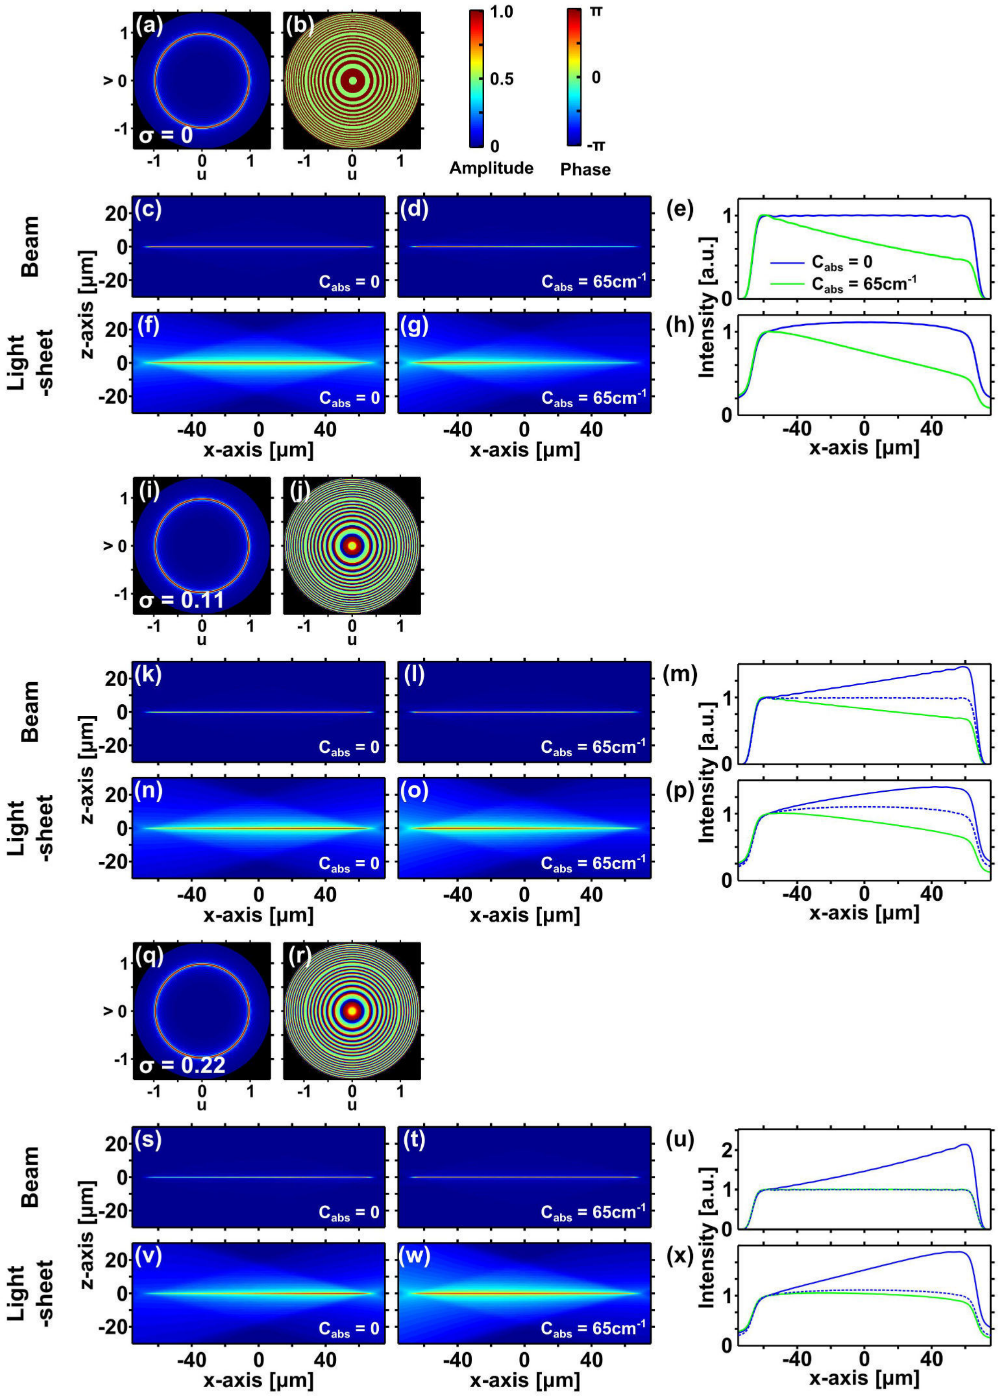


Figure S6: Amplitude (a,i,q) and phase (b,j,r) pupil functions, corresponding Bessel beam profiles in free-space (c,k,s) and in an absorbing medium (d,l,t) with $C_{abs} = 65\text{cm}^{-1}$ (on-axis profiles (e,m,u)), and corresponding light-sheet profiles (f-h,n-p,v-x) for $\sigma = 0$ (a-h), $\sigma = 0.11$ (i-p), $\sigma = 0.22$ (q-x). Additional parameters: $\beta = 0.05$, $\lambda = 532$nm, NA $= 0.42$, and $n = 1.33$. Pupil amplitudes have been normalised to their maximum value for display.

# S3 Modification of deconvolution protocol incorporating attenuation and attenuation-compensation

The following Note describes modifications to the Airy light-sheet microscopy deconvolution strategy required to incorporate attenuation-compensated beams and attenuation. The original deconvolution strategy is described by Vettenburg *et al* [11].

### Airy light-sheet microscopy deconvolution strategy

The recorded image stack can be considered as a convolution of the specimen fluorophore distribution with the light-sheet profile. The light-sheet profile dictates only the axial resolution but is spatially-variant along the propagation axis of the illumination. Therefore, a 1D spatially-variant Wiener filter is suitable to deconvolve the recorded image stack, given by:

$$H_W(x,\nu_z) = \frac{H(x,\nu_z)^*}{|H(x,\nu_z)|^2 + SNR(\nu_z)^{-2}} \tag{S22}$$

where $H(x,\nu_z) = \mathcal{F}_z[LS(x,z)]$ is the 1D optical transfer function (OTF; Fourier transform) in $z$ of the light-sheet profile, $LS(x,z)$, $SNR(\nu_z) = k\nu_{cut-off}/\nu_z$ is related to the signal-to-noise of the recorded images, modelled as a power law distribution, where $k$ is a filter constant (typically $k = 5$) and $\nu_{cut-off} = 2\text{NA}/\lambda$ where NA and $\lambda$ are the numerical aperture and wavelength of the light-sheet respectively. To prevent edge artefacts in the deconvolution process, the light-sheet profile is zero-padded in $z$ to double its axial dimension before calculation of the OTF.

The deconvolved image stack ($I_{dec}(x,y,z)$) is then determined by multiplication of the 1D Fourier transform along the $z-$axis of the image stack ($\tilde{I}_{rec}(x,y,\nu_z) = \mathcal{F}_z[I_{rec}(x,y,z)]$) with the Wiener filter ($H_W(x,\nu_z)$) and taking the 1D inverse Fourier transform along the $z-$axis to return this to real-space coordinates, given by:

$$I_{dec}(x,y,z) = \mathcal{F}^{-1}_{\nu_z}[\tilde{I}_{rec}(x,y,\nu_z) \cdot H_W(x,\nu_z)] \tag{S23}$$

Again, before taking the Fourier transform of $I_{rec}(x,y,z)$, the first and last frames of the image stack are replicated in order to double its axial dimension and reduce the potential impact of deconvolution artefacts. After deconvolution, $I_{dec}(x,y,z)$ is cropped to the size of the original image stack to remove the replicated frames.

### Determination of attenuation-compensated light-sheet profile

The only modifications required to deconvolve image stacks acquired with attenuation-compensated Airy light-sheets are the determination of the light-sheet profile, $LS(x,z)$, and the relative weighting of its OTF, $H(x,\nu_z)$.

The light-sheet profile, $LS(x,z)$, is determined by generating a 3D model of the attenuation-compensated Airy beam in the sample, and integrating this along the $y-$axis to yield the light-sheet profile. The beam profile is determined from the Fourier transform of the pupil function given by (S7) and propagated along the $x-$axis by multiplying the pupil function by a defocus term given by:

$$P_{defocus}(u,v) = \exp(2\pi i d[u^2+v^2]) \tag{S24}$$

where $d$ is a defocus parameter related to the physical longitudinal displacement, $\Delta x$, by:

$$d = \Delta x \frac{n}{\lambda}\left(1 - \sqrt{1 - \left(\frac{\text{NA}}{n}\right)^2}\right) \tag{S25}$$

where $n$ is the refractive index of the sample medium.

The light-sheet profile must be determined at $x-$ and $z-$coordinates corresponding to the $x-$ and $z-$pixel locations in the recorded image stack. As the beam profile is integrated along the $y-$axis to determine the light-sheet profile, accurate pixel-registration along the $y-$axis is not critical and can simply be Nyquist sampled.

The light-sheet profile is then modulated by a Gaussian envelope along the $z-$axis with width given by the depth-of-field (DOF) of the detection objective lens to suppress contributions from the light-sheet profile that generate fluorescence outwith the DOF and not contributing to signal.

To model attenuation, the light-sheet profile is further modulated by an exponential ($\exp(-C^D_{attn}x)$), where $C^D_{attn}$ is the estimate of $C_{attn}$ used in the deconvolution process.

The OTF of the attenuated light-sheet profile is then determined from the 1D Fourier transform along the $z-$axis as described above. This is typically normalised such that $|H(0,0)| = 1$. To account for the additional energy delivered by the light-sheet when using attenuation-compensation, the OTF was normalised such that $|H(0,0)| = 1$, and then multiplied by an additional scaling factor, $A_{OTF}(\sigma)$, given by:

$$A_{OTF}(\sigma) = \frac{A^2_\sigma \exp(-2\sigma)}{A^2_0} \tag{S26}$$

where $A_\sigma$ is a pupil amplitude scaling factor described in Supp. Note S1.

Deconvolution was then performed as described above using the weighted OTF.

## S4 Theoretical imaging performance of attenuation-compensated Airy beam light-sheet

The following Note discusses the effect of attenuation and attenuation-compensation on Airy beam light-sheet imaging.

Resolution can be considered in the Fourier domain, where the definition of resolution changes from the smallest resolvable feature to the largest resolvable spatial frequency. This definition of resolution is particularly useful when considering imaging methods which utilise deconvolution, such as Airy light-sheet microscopy [11]. In theory the resolution is given by the greatest spatial frequency with non-zero magnitude; however, in practice this depends on the experimental noise floor, and the resolution is given by the greatest spatial frequency which can be distinguished from noise. By this definition, resolution and signal-to-noise ratio (SNR) are intrinsically linked.

To investigate the effect of attenuation and attenuation-compensation on the imaging performance of Airy light-sheet microscopy, we study the axial modulation transfer function (MTF) of the light-sheet cross section across the field-of-view (FOV). The MTF is the absolute magnitude of the optical transfer function (OTF), also known as the Fourier transform of the point spread function (PSF). The MTF reveals the spatial frequency content that the light-sheet can successfully capture in an image.

Figure S7 shows the effect of attenuation and attenuation-compensation on an Airy light-sheet ($\alpha = 7$). Fig. S7(a) shows the standard Airy light-sheet propagating in a medium with no absorption. The 5% threshold of the axial MTF of this light-sheet is shown in Fig. S7(b). Assuming a noise floor at 5%, this threshold indicates the maximum spatial frequency which can be resolved by the light-sheet. The unattenuated, uncompensated 5% threshold is shown as a green dashed line in subsequent MTF plots for comparison.

Figs. S7(c-l) show light-sheets (left-hand column) and corresponding MTFs (right-hand column) for the same Airy light-sheet as in (a) in a medium with absorption coefficient $C_{abs} = 64.95$ cm$^{-1}$ and varying degrees of compensation. $C_{abs} = 64.95$cm$^{-1}$ is the maximum attenuation that can be fully compensated for an Airy light-sheet with $\alpha = 7$ (see Supp. Note S1). Figs. S7(c,d) show the case of no compensation ($\sigma = 0$). There is visible attenuation of the light-sheet intensity across the FOV, and the MTF becomes asymmetric and attenuated, indicating a loss in achievable resolution, particularly to the right of the focal position (at greater depths). The red dashed lines in subsequent MTF plots indicates the 5% threshold as shown in Fig. S7(d) for comparison. Figs. S7(e-l) show cases with $\sigma = 0.1$, $\sigma = 0.3$, $\sigma = 0.5$ (partial compensation), and $\sigma = 0.54$ (full compensation), respectively. For $\sigma = 0.3$ and up, the MTF shows that the compensated light-sheet achieves the same or higher resolution across the FOV as the uncompensated light-sheet in a non-absorbing medium.

Fig. S7(m) shows the maximum transverse intensity of the light-sheets along the propagation axis. It shows that $\sigma = 0.54$ perfectly restores the light-sheet intensity across the FOV. Fig. S7(n) shows the relative pupil amplitude functions which generate the light-sheets shown in Figs. S7(a-l).

While the 5% threshold of the MTF is indicative of resolution, it is not definitive. For example, Fig. S7(b) indicates that the standard Airy light-sheet with the parameters shown should have resolution of about one tenth the maximal achievable resolution at a longitudinal distance of $\pm 150$ µm away from focus (approximately 10 µm for the simulation parameters). This is in contrast to the findings of Vettenburg *et al* [11], which showed experimentally that an Airy light-sheet microscope with the same parameters can yield an axial resolution of approximately 2 µm at the same distance. The simulations shown in Fig. S7 indicate that a reduction in image quality, a combination of reducing SNR and reducing resolution, is to be expected as the light-sheet propagates into specimens which attenuate the light-sheet, and that the use of attenuation-compensation can recover the lost intensity and increase the axial resolution.

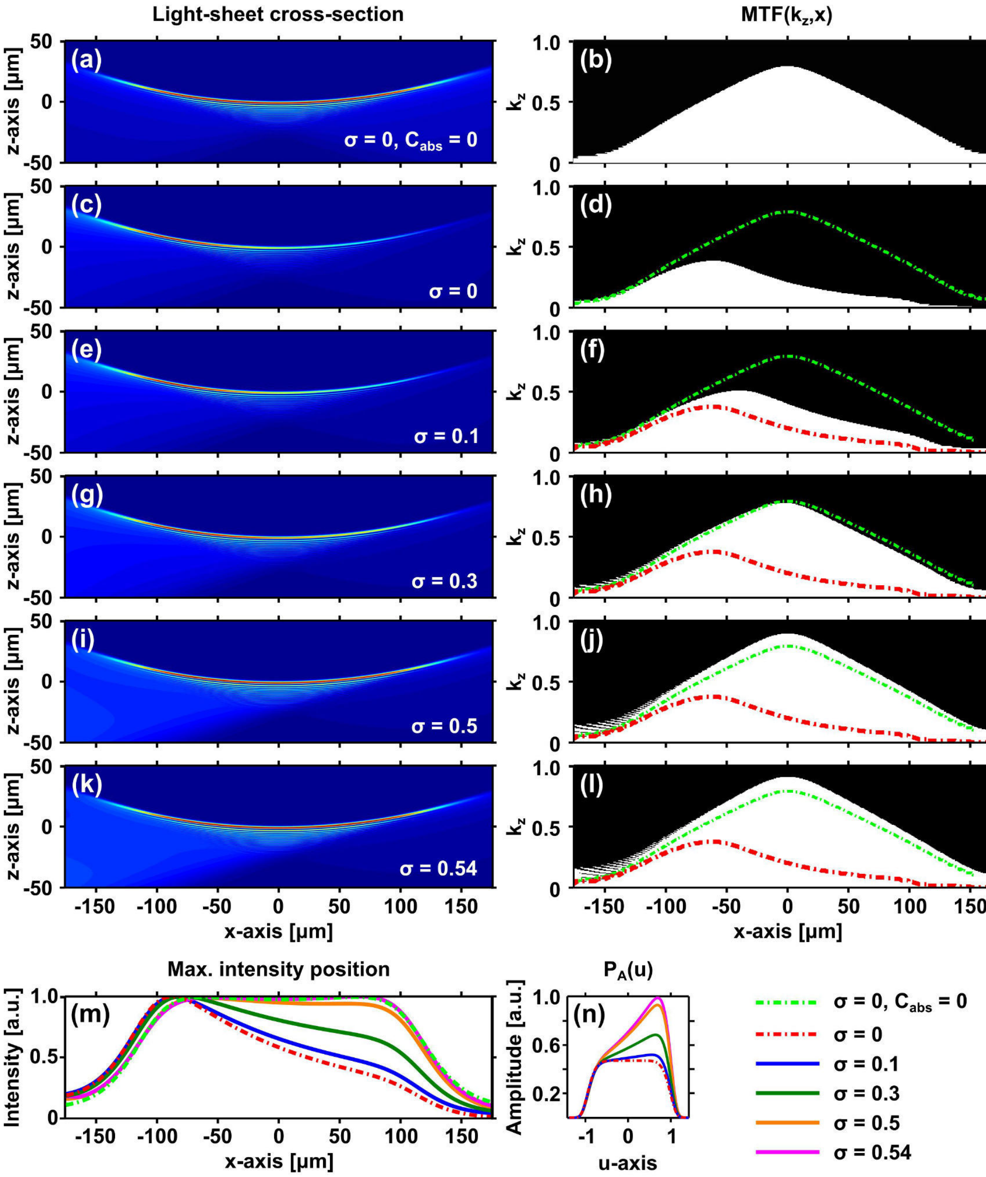


Figure S7: (a-l) Simulated attenuation-compensated Airy light-sheet profiles (left) and corresponding MTFs (right; thresholded at 5%) shown for an Airy light-sheet ($\alpha = 7$) without and with attenuation (top and $2^{nd}$ rows respectively), and with various degrees of compensation ($3^{rd} - 6^{th}$ rows). (m) Normalised longitudinal intensity profiles and (n) pupil functions for each light-sheet shown.

# S5 Effect of incorrect attenuation estimation on deconvolution

The following Note discusses the effects on the deconvolution of Airy LSM images caused by incorrect estimation of the sample attenuation.

In addition to determining the necessary degree of attenuation-compensation, precise knowledge of the attenuation profile is crucial for determining an accurate light-sheet PSF in an attenuating medium, which in turn is necessary for accurate deconvolution (see Supp. Note S3).

Here we consider error from the point of view of accurate deconvolution. Fig. 1 in the Main Text shows simulated images of the University Crest imaged with various degrees of attenuation-compensation in a linearly absorbing medium ($C_{attn} = 64.95\text{cm}^{-1}$). During the deconvolution process, the light-sheet profile as it would appear in free-space is modulated by an exponential function ($\exp(C^D_{attn}x)$) to model attenuation, where $C^D_{attn}$ is the estimate of $C_{attn}$ used for deconvolution. The images shown in Fig. 1 have been deconvolved with the correct attenuation coefficient ($C^D_{attn} = C_{attn} = 64.95\text{cm}^{-1}$). However, if the estimate for the attenuation coefficient, $C^D_{attn}$, deviates from the true attenuation, $C_{attn}$, then the deconvolved image will contain artefacts.

Figure S8 shows simulated images of the same recorded data shown in Fig. 1(k,n) ($C_{attn} = 64.95\text{cm}^{-1}$, $\sigma = 0$) with an error in $C^D_{attn}$ of ±10%, ±50%, and ±100% $C_{attn}$. Figure S8(d) repeats the $C^D_{attn} = C_{attn}$ case for comparison.

Figure S9 shows simulated images of the same recorded data shown in Fig. 1(l,o) ($C_{abs} = 64.95\text{cm}^{-1}$, $\sigma = 0.54$) with the same error in $C^D_{attn}$. Again, Fig. S9(d) shows the case of correct deconvolution.

Both figures show that the deconvolution artefacts resulting from incorrect estimation of specimen attenuation are essentially negligible if the magnitude of the error is below 10% $C_{attn}$. However, even in the absence of compensation, large underestimates of the sample attenuation shift the peak intensity towards the left of the image, whereas overestimates shift it towards the right. When $C^D_{attn}$ matches the sample attenuation, the image intensity is fairly uniform across the FOV. This can be understood because the deconvolution utilises knowledge of the light-sheet PSF, including knowledge of its intensity as it propagates, to restore the sample fluorophore distribution.

Errors in $C^D_{attn}$ also introduce errors in the estimate of the light-sheet OTF. As discussed in Supp. Note S4, attenuation of the Airy light-sheet reduces the MTF, and therefore the maximal achievable axial resolution. If the attenuation is underestimated, the MTF will be overestimated, and noise will be amplified as the light-sheet propagates. If the attenuation is overestimated, the MTF will be underestimated, and high spatial frequency details will be rejected from the image as noise. Underestimation of the MTF effectively leads to excessive axial low-pass filtering of the image, as observed in Fig. S8(e-g) and S9(e-g).

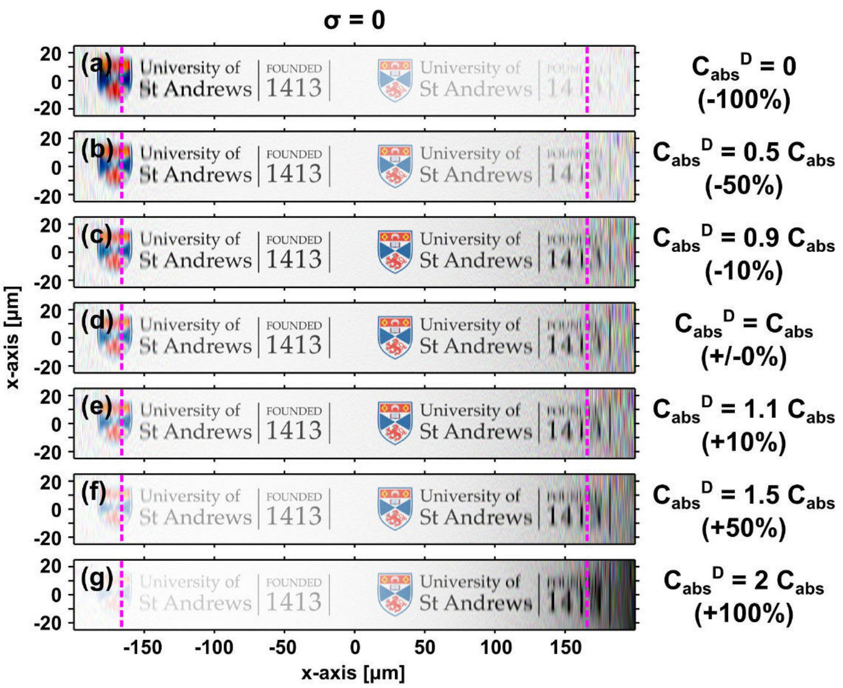


Figure S8: Simulated images of University Crest imaged by standard Airy LSM ($\sigma = 0$) in absorbing medium ($C_{abs} = 64.95\text{cm}^{-1}$) with ±10%, ±50%, and ±100% error in the estimation of the sample attenuation.

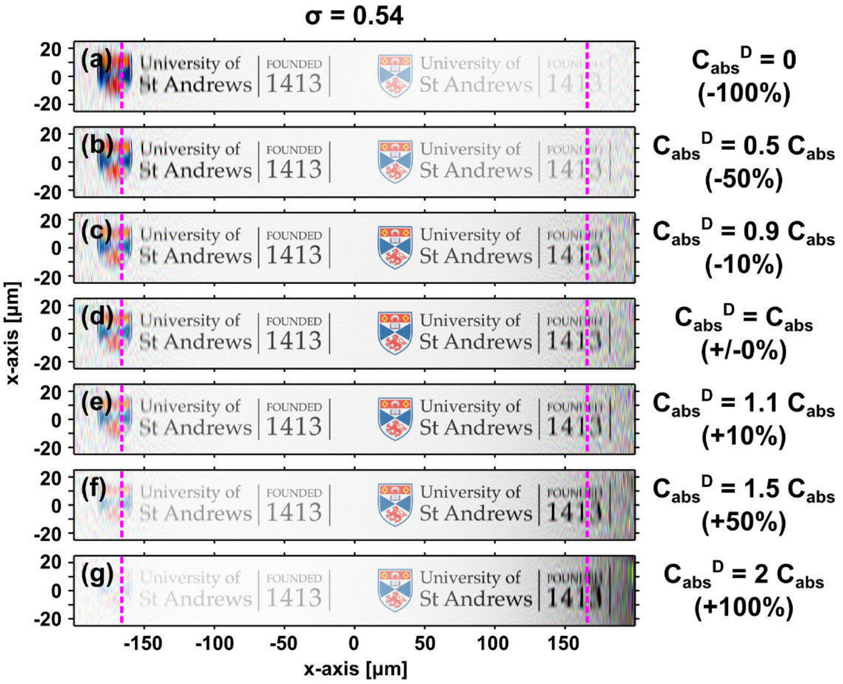


Figure S9: Simulated images of University Crest imaged by attenuation-compensated Airy LSM ($\sigma = 0.54$) in absorbing medium ($C_{abs} = 64.95\text{cm}^{-1}$) with ±10%, ±50%, and ±100% error in the estimation of the sample attenuation.

# S6 Theoretical imaging performance of attenuation-compensated Bessel beam light-sheet

The following Note discusses the effect of attenuation and attenuation-compensation on Bessel beam based light-sheet imaging modalities.

Unlike Airy-beam light-sheets, Bessel beam imaging methods typically do not utilise deconvolution, and so it is more informative to consider the effects of attenuation and attenuation-compensation in real-space rather than Fourier space, in terms of the effect on the PSF of the light-sheet.

We compared the $z-$axis cross-sectional beam and light-sheet profiles with attenuation-compensation to those without any compensation, as determined from simulations. Due to the changing intensity on propagation of the attenuation-compensated beams, each cross-sectional profile was scaled to minimise the difference (error) between profiles. We define the cross-sectional PSF error as:

$$Error(z) = I_0(z) - AI_\sigma(z) \tag{S27}$$

where $I_\sigma(z)$ is the $z-$axis cross-sectional profile of the beam with compensation parameter, $\sigma$. $A$ is a scaling factor that accounts for the additional intensity of the attenuation-compensated beam but does not affect its cross-sectional shape.

Figure S10(a-j) and S11(a-j) show cross-sectional profiles through the Bessel beams shown in Fig. S6(c,k,s) and their mutual error. Figure S10(k) and S11(k) also show the root-mean-squared error (RMSE) for each cross-section as a function of propagation coordinate. Both Figures show that the error between the compensated (green/red) and non-compensated (blue) beam shapes is very small (note the scaling by $10^{-4}$ or $10^{-3}$ in Fig. S10(f-k) and S11(f-k)). The deviation in shape is, on average, less than 0.5% everywhere in the beam. The evolution of the RMSE with propagation also reveals that there is more deviation from the non-compensated profile before reaching focus ($x = 0$) than after focus. This is expected as the additional energy delivered into the beam to achieve attenuation-compensation is delivered along trajectories that originate off-axis, contributing a broad off-axis signal, then progressing towards the on-axis region of the beam where these rays contribute positively for formation of the beam profile.

Figure S12 and S13 show similar plots for the light-sheets these Bessel beams generate (shown in Fig. S6(f,n,v)). These Figures show that there is much more deviation in shape for the light-sheets than in the beams themselves. Figure S12(f-j) and S13(f-j) show that the error can reach nearly 10% for $\sigma = 0.11$ and 20% for $\sigma = 0.22$. The RMSE on propagation (Fig. S12(k) and S13(k)) shows that the deviation in shape with attenuation is, on average, less than 4% everywhere in the light-sheet. This is a much greater deviation than for the static beams, but still relatively low.

These simulations show that the effect of attenuation-compensation on the cross-sectional shape of a Bessel beam is small. In all simulations, attenuation-compensation did not affect the full-width at half-maximum (FWHM) of the Bessel beam core, which maintained a constant value of 460nm. As the beam shape remains effectively unaltered, attenuation-compensation is expected to to be complimentary to light-sheet imaging techniques exploiting stepped Bessel beams [33,34] or arrays of Bessel beams [16–18].

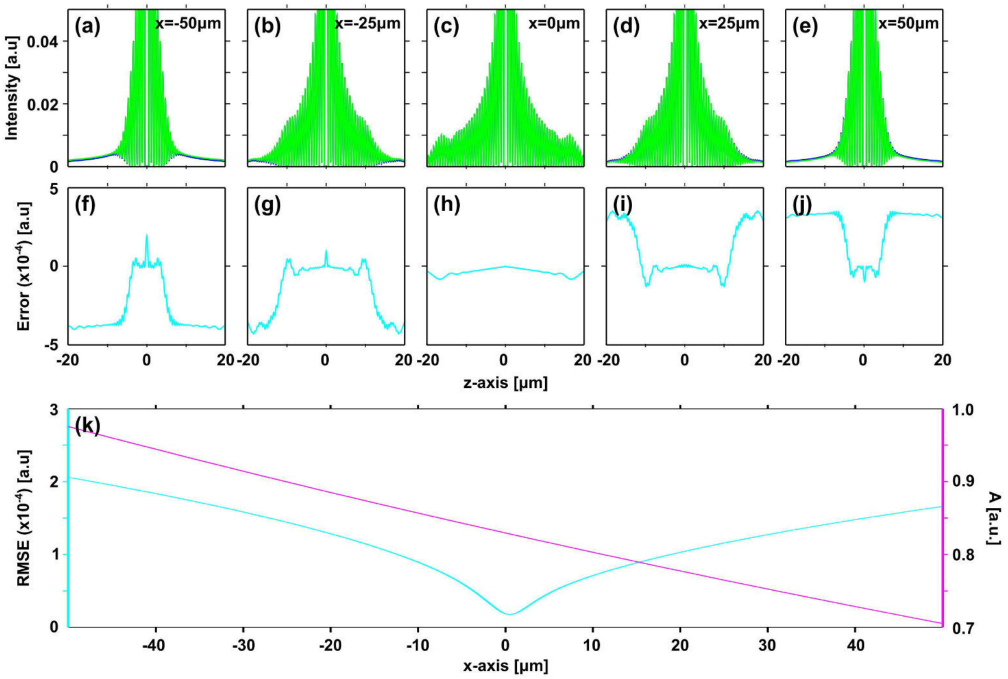


Figure S10: Comparison of Bessel beam transverse profiles without and with attenuation-compensation ($\sigma = 0.11$). $z-$axis cross-sectional beam profiles through $y = 0$ and (a) $x = -50\,\mu m$, (b) $x = -25\,\mu m$, (c) $x = 0\,\mu m$, (d) $x = 25\,\mu m$, (e) $x = 50\,\mu m$ for non-compensated (blue) and compensated (green) Bessel beams. (f-j) Corresponding PSF error given by (S27) for profiles shown in (a-e). (k) RMS error as a function of the beam propagation axis (cyan) and the fitted scaling factor, $A$ (magenta).

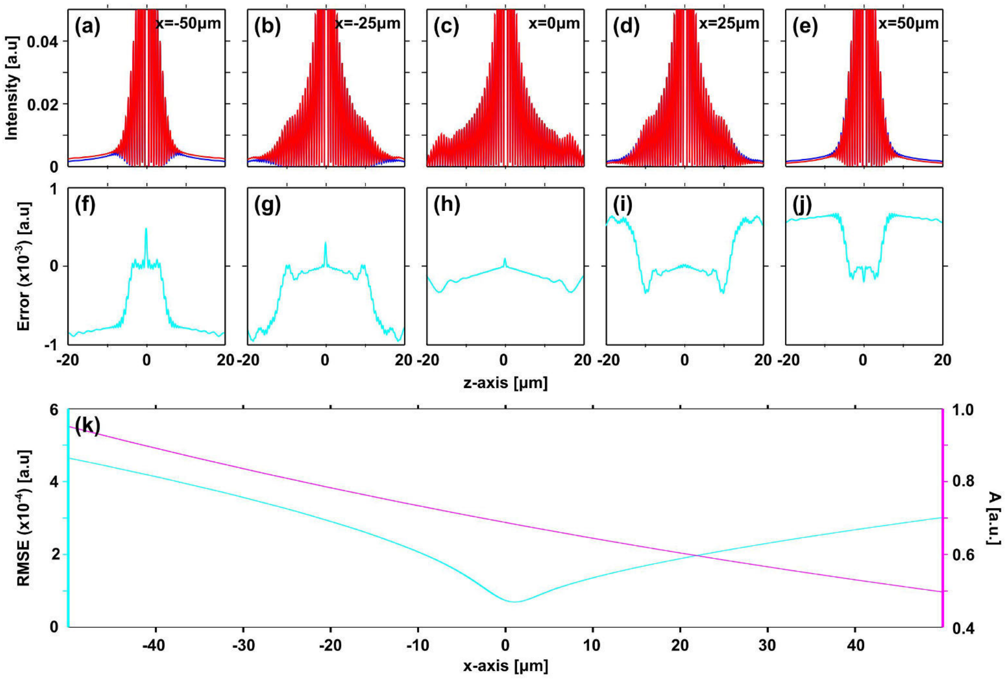


Figure S11: Comparison of Bessel beam transverse profiles without and with attenuation-compensation ($\sigma = 0.22$). $z-$axis cross-sectional beam profiles through $y = 0$ and (a) $x = -50\,\mu m$, (b) $x = -25\,\mu m$, (c) $x = 0\,\mu m$, (d) $x = 25\,\mu m$, (e) $x = 50\,\mu m$ for non-compensated (blue) and compensated (red) Bessel beams. (f-j) Corresponding PSF error given by (S27) for profiles shown in (a-e). (k) RMS error as a function of the beam propagation axis (cyan) and the fitted scaling factor, $A$ (magenta).

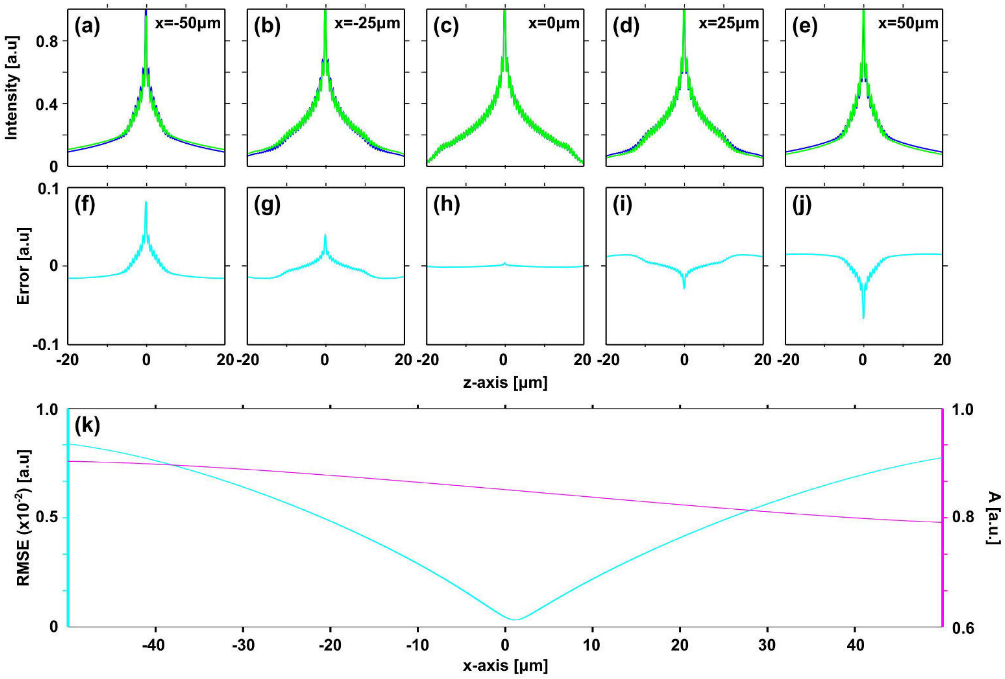


Figure S12: Comparison of Bessel light-sheet transverse profiles without and with attenuation-compensation ($\sigma = 0.11$). $z-$axis cross-sectional light-sheet profiles through $y = 0$ and (a) $x = -50\,\mu m$, (b) $x = -25\,\mu m$, (c) $x = 0\,\mu m$, (d) $x = 25\,\mu m$, (e) $x = 50\,\mu m$ for non-compensated (blue) and compensated (green) Bessel beams. (f-j) Corresponding PSF error given by (S27) for profiles shown in (a-e). (k) RMS error as a function of the light-sheet propagation axis (cyan) and the fitted scaling factor, $A$ (magenta).

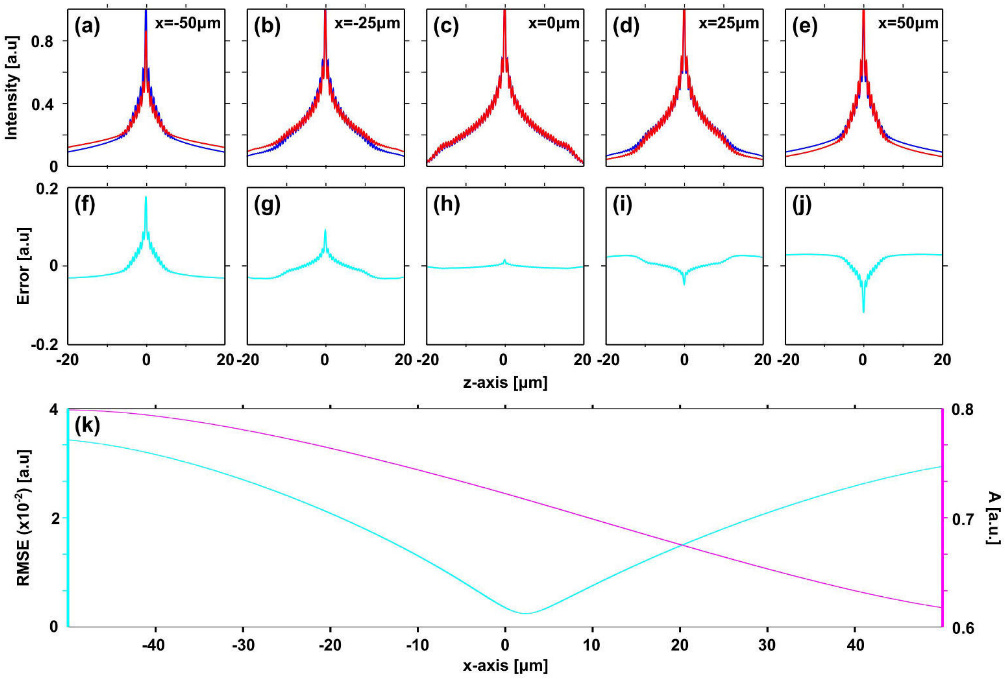


Figure S13: Comparison of Bessel light-sheet transverse profiles without and with attenuation-compensation ($\sigma = 0.22$). $z-$axis cross-sectional light-sheet profiles through $y = 0$ and (a) $x = -50\,\mu m$, (b) $x = -25\,\mu m$, (c) $x = 0\,\mu m$, (d) $x = 25\,\mu m$, (e) $x = 50\,\mu m$ for non-compensated (blue) and compensated (red) Bessel beams. (f-j) Corresponding PSF error given by (S27) for profiles shown in (a-e). (k) RMS error as a function of the light-sheet propagation axis (cyan) and the fitted scaling factor, $A$ (magenta).

# S7 Determination of specimen attenuation

The following Note discusses strategies for determining the attenuation of a specimen in order to achieve effective and correct attenuation-compensation.

In the attenuating phantom seeded sparsely with fluorescent beads (Fig. 2), the background is weakly fluorescent. A mean projection over a data volume will be dominated by the background signal, which decays with attenuation and therefore can be accurately fit to give the absorption coefficient.

In a non-fluorescent attenuating phantom or a biological specimen (Fig. 3 - 5), the signal as a function of depth in the data cube will depend on the density and distribution of fluorophores as well as the attenuation, so a mean projection cannot be used to estimate the absorption coefficient. We found that it was necessary to perform a maximum value projection and estimate the attenuation on a per-image basis. Depending on the uniformity of the sample, it may be necessary to perform this procedure per-image or simply per-sample. We assumed exponential intensity decay across the image, and divided the image by a decaying exponential as a function of $x-$axis coordinate. The attenuation was determined to be the decay parameter which yielded approximately uniform intensity structures throughout the image after division.

## S8 Sample-based geometric effects on attenuation

The following Note discusses the effects of specimen geometry on the attenuation profile of the light-sheet.

In a microscope with collinear illumination and detection, the intensity of fluorescence signal at any point in the specimen is given by the Beer-Lambert law:

$$I_{Fluor}(r) = \exp[-C_{attn} r] \tag{S28}$$

where $C_{attn}$ is the attenuation coefficient, which we assume to be constant for simplicity, and $r$ is the specimen thickness (in transillumination) or the imaging depth (in epi-illumination).

In the case of light-sheet microscopy, the orthogonal illumination and detection pose additional geometric challenges for attenuating specimens. The observed attenuation profile will be the product of the light-sheet attenuation profile and the spatially-variant attenuation of the generated fluorescence.

The simplest case is a sample with a square cross section, with illumination and detection pathways parallel to two sides of the square (Fig. S14(a)). The attenuation profile of the light-sheet is exponential on propagation, and the fluorescence attenuation profile is constant across the FOV. Therefore the fluorescence intensity is given by:

$$I_{Fluor}(x) \propto \exp[-C_{attn} x] \tag{S29}$$

In the case of tissue slices oriented at 45° to both illumination and detection pathways (Fig. S14(b)), the attenuation of the fluorescence signal at any point across the FOV is equal to the attenuation of the light-sheet at that point by symmetry. Therefore the total fluorescence intensity is given by:

$$I_{Fluor}(x) = \exp[-2C_{attn} x] \tag{S30}$$

Embryonic or spheroidal specimens will have a circular cross section (Fig. S14(c)). The flat plane of the light-sheet and the circular edge of the specimen result in the spatially-variant fluorescence intensity given by:

$$I_{Fluor}(x) = \exp[-C_{attn}(x + R\sin(\pi x/2R))] \tag{S31}$$

where $R$ is the radius of the specimen cross section.

Figure S14(d) summarizes the profiles given by (S29) - (S31). The additional optical path length when imaging in tissue sections causes a more rapid attenuation of the fluorescence across the FOV, as if the attenuation has effectively doubled). The morphology of spheroidal tissue results in a more complex attenuation profile. As the light-sheet propagates from the initial edge of the specimen ($x_0$) to its centre the attenuation is rapid (approximating an exponential decay with coefficient greater than twice the standard specimen attenuation coefficient). From the centre to the far edge, the rate of attenuation decreases, and the intensity even increases slightly at the far edge.

In this study, we have only simulated attenuation according to the linear, constant-attenuation model in equation S29. We have used the linear constant-attenuation profiles S29 and S30 to model attenuation in the specimens discussed in the Main Text. The fluorescent beads in attenuating phantom (Section 2.2) were prepared in a glass square-walled capillary tube and oriented as in S14(a). Attenuation in the mouse brain tissue slice discussed in Section 2.3 was described by equation (S30). The *S. lamarcki* opercula imaged in Section 2.3 can be considered 'quasi-circular' in cross-section but since the effective radius is larger than the FOV of the microscope, it could also be modelled using equation (S29) rather than equation (S31). However, the principle of attenuation is more general than linear attenuation and can be used to counteract any decay profile. Indeed, an important future step will be to determine accurate real-time methods to model and correct for arbitrary decay profiles in dynamic specimens.

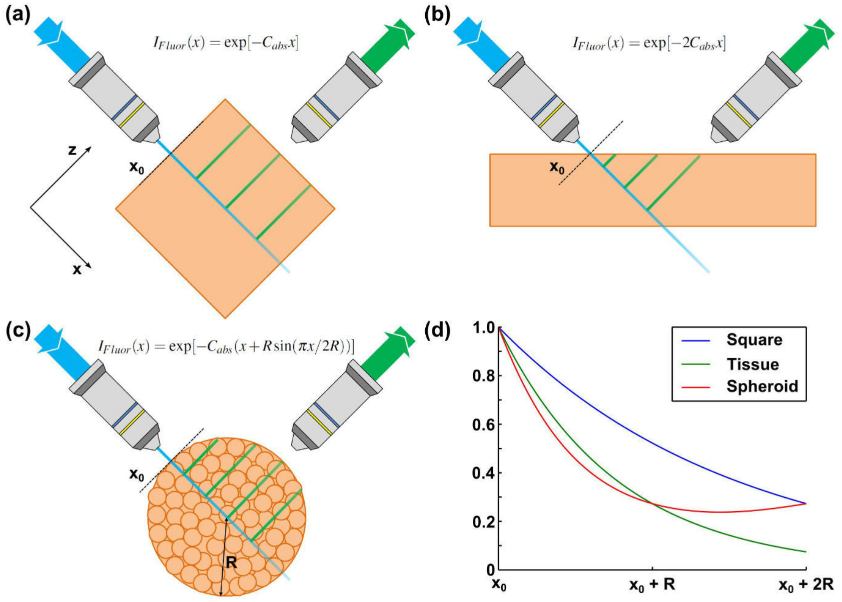


Figure S14: Illustrations of different sample geometries in LSM (a-c) and the intensity decay expected across the image for each geometry (d).

# S9 Attenuation-compensation of multi-photon excitation Airy and Bessel light-sheets

The following Note discusses the attenuation and attenuation-compensation of two-photon excitation (2PE) schemes in Airy and Bessel beam-based light-sheet imaging.

Using the framework for attenuation-compensation described in Supp. Notes S1 and S2, we extend our analysis to consider the effects of attenuation and attenuation-compensation on 2PE light-sheet microscopy. 2PE is a non-linear optical process, and its efficiency scales with the square of the illumination intensity. As highlighted in Supp. Notes S2 and S6, there are differences in the performance of Bessel beam light-sheet imaging modes dependent on whether the beam is swept rapidly or discretely stepped. In the non-linear regime, there are also subtle differences in the generation of an Airy light-sheet, dependent on whether a 1+1D Airy beam is used in conjunction with a cylindrical lens, or if a 2+1D Airy beam is used in conjunction with rapid, single-axis scanning. Here, we consider all 4 scenarios for completeness.

The 2PE cross-section of an Airy light-sheet formed by cylindrical focusing of a 1+1D Airy beam depends on the intensity distribution of the illuminating light-sheet. By contrast, when the light-sheet is formed by digital scanning of a 2+1D Airy beam, the 2PE cross-section is defined by the intensity distribution of the beam. Scanning of this 2PE beam cross-section gives the 2PE cross-section of the light-sheet as a whole. Likewise, the 2PE cross-section of a stepped Bessel beam is simply the square of the intensity of the illuminating Bessel beam, while the 2PE cross-section of a digitally scanned Bessel beam light-sheet is the integral of the 2PE beam cross-section along the scan axis.

For each scenario, the relevant beam or light-sheet profile was simulated for the centre wavelength of the illumination (800nm); the effect of attenuation (absorption) was applied to the illumination; and then the 2PE cross-section was determined from the resulting intensity profile. Beam parameters were adjusted to give equivalent FOV and attenuation-compensation properties to the single-photon excitation simulations shown in earlier Sections. In all four cases, the effect of under-compensated attenuation has a much more dramatic effect on the effective FOV of the 2PE signal due to the non-linear dependence of the 2PE cross-section on illumination intensity, as summarized in Tables S1 and S2.

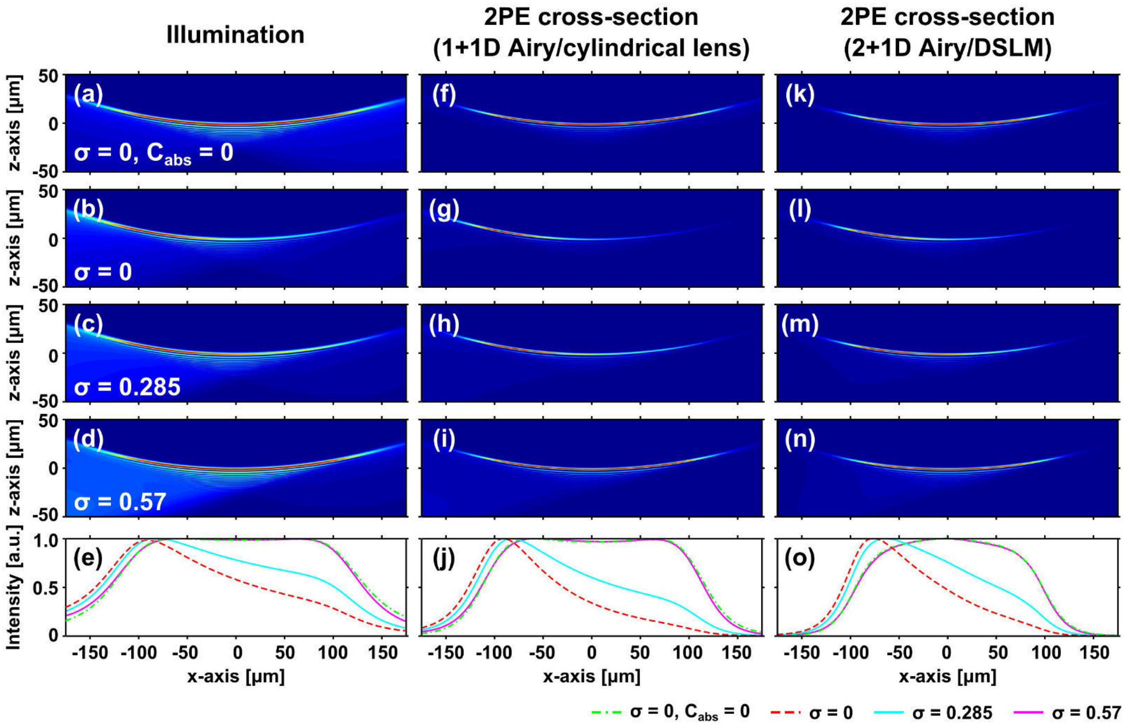


Figure S15: Illumination profiles (a-d) of attenuation-compensated 2PE Airy light-sheets and their corresponding 2PE cross-sections for light-sheets formed by a 1+1D Airy beam and a cylindrical lens (f-i) and by a 2+1D Airy beam and digital scanning (k-n) for no attenuation and no compensation (top row), attenuation ($C_{abs} = 65\text{cm}^{-1}$) and no compensation (2nd row), partial compensation (3rd row), and full compensation (4th row). Peak transverse intensity profiles for the illumination, and 2PE cross sections are shown in (e,j,o) respectively. The illumination cross-section (a-e) does not depend on the method of light-sheet generation.

## 2PE Airy light-sheet microscopy with a 1+1D Airy SPIM

Figure S15(a-d) show the intensity profiles of 1+1D Airy light-sheets with a centre wavelength of 800nm, $\alpha = 5$, and various degrees of attenuation-compensation. For this light-sheet, $\sigma = 0.57$ allowed compensation of $C_{abs} = 65\text{cm}^{-1}$ attenuation. Figure S15(f-i) show the associated 2PE cross-sections for these light-sheets, and Fig. S15(e,j) show the transverse peak intensity of the light-sheets on propagation.

## 2PE Airy light-sheet microscopy with a 2+1D Airy DSLM

Figure S15(k-n) show the 2PE cross-sections of light-sheets formed by digital scanning. The parameters are the same as for as their cylindrically focused counterparts shown in Fig. S15(f-i). The illumination intensity profiles are the same for both light-sheet generation methods (Fig. S15(a-d)). Like the 1+1D 2PE Airy light-sheet, the FOV of the 2+1D light-sheet is severely affected by under-compensation (Fig. S15(o)).

| $C_{abs}[\text{cm}^{-1}]$ | $\sigma$ | FOV [μm] (1+1D Airy-SPIM) | FOV [μm] (2+1D Airy-DSLM) |
|---|---|---|---|
| 0 | 0 | 230 | 192 |
| 65 | 0 | 98 (43%) | 103 (54%) |
| 65 | 0.285 | 150 (65%) | 155 (81%) |
| 65 | 0.57 | 230 (100%) | 192 (100%) |

Table S1: Airy 2PE FOV given by the longitudinal FWHM for SPIM- and DSLM-style systems with various degrees of attenuation and attenuation-compensation. The percentage in brackets is the FOV relative to the case of no attenuation.

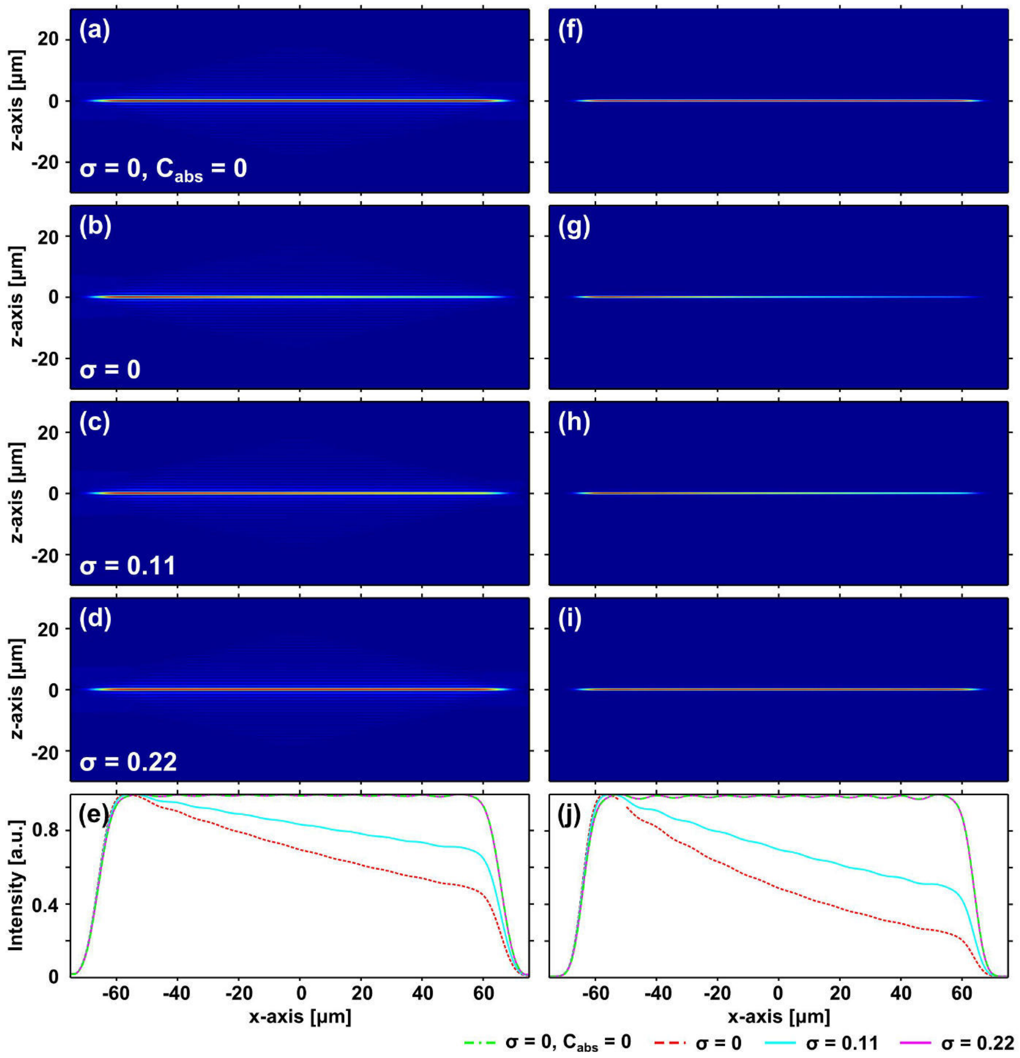


Figure S16: Illumination profiles (a-d) of attenuation-compensated 2PE Bessel beams and their corresponding 2PE cross-sections (f-i) for no attenuation and no compensation (top row), attenuation ($C_{abs} = 65\text{cm}^{-1}$) and no compensation (2nd row), partial compensation (3rd row), and full compensation (4th row). On-axis intensity profiles for the illumination, and 2PE cross sections are shown in (e,j) respectively.

## 2PE Bessel beam light-sheet microscopy with a stepped Bessel beam

Figure S16(a-d) shows the intensity profile of the illuminating, stepped Bessel beam with centre wavelength of 800nm, $\beta = 0.75$, and various degrees of attenuation-compensation. For this beam, $\sigma = 0.22$ allowed compensation of $C_{abs} = 65\text{cm}^{-1}$ attenuation. Figure S16(f-i) shows the associated 2PE cross-sections of these beams, and Fig. S16(e,j) show the on-axis profiles of these beams on propagation. Again, the effect of under-compensation of attenuation is more pronounced on the 2PE cross-section than on the illumination profile.

## 2PE Bessel beam light-sheet microscopy with a digitally scanned Bessel beam

The 2PE cross-section of a digitally scanned Bessel beam light-sheet is the integral of the 2PE beam cross-section along the scan axis (Fig. S17(a-d)). Figure S17(f-i) shows the 2PE light-sheet cross-sections of the Bessel beams shown in (a-d), and Fig. S17(e,j) show the on-axis profiles of these light-sheets on propagation.

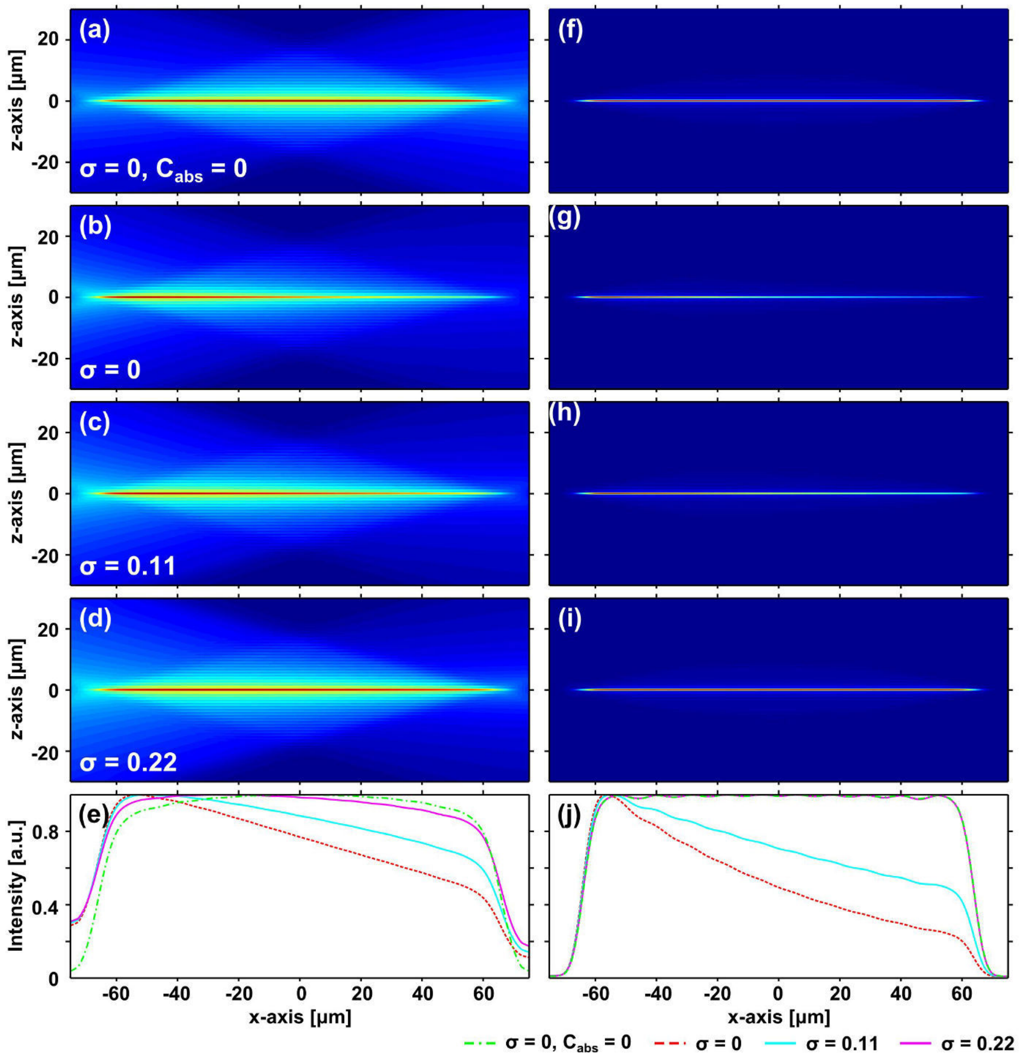


Figure S17: Illumination profiles (a-d) of attenuation-compensated 2PE Bessel light-sheets and their corresponding 2PE cross-sections, formed by digital scanning of the beams shown in Supp. Fig. S16, for no attenuation and no compensation (top row), attenuation ($C_{abs} = 65\text{cm}^{-1}$) and no compensation (2nd row), partial compensation (3rd row), and full compensation (4th row). On-axis intensity profiles for the illumination, and 2PE cross sections are shown in (e,j) respectively.

| $C_{abs}[\text{cm}^{-1}]$ | $\sigma$ | FOV [μm] (Bessel beam) | FOV [μm] (Bessel-sheet) |
|---|---|---|---|
| 0 | 0 | 127 | 127 |
| 65 | 0 | 62.5 (49%) | 62.5 (49%) |
| 65 | 0.285 | 117 (92%) | 117 (92%) |
| 65 | 0.57 | 127 (100%) | 127 (100%) |

Table S2: Bessel 2PE FOV given by longitudinal FWHM for Bessel beams (Fig. S16) and Bessel-sheets (Fig. S17) with various degrees of attenuation and attenuation-compensation. The percentage in brackets is the FOV relative to the case of no attenuation.

# S10 Additional Supplementary Figures and Tables

The following Supplementary section contains additional Supplementary Figures and Tables and their descriptions. Each Figure or Table is given a separate page.


| **Fig. #** | **Description** | **Page #** |
|---|---|---|
| S18 | Simulated images of a 1D resolution target with/without attenuation and attenuation-compensation. | S25 |
| S19 | Line profiles through simulated images of a 1D resolution target shown in Fig. S18. | S26 |
| S20 | Local SBR and CNR measured for data shown in Fig. 3. | S27 |
| S21 | Local SBR and CNR measured for data shown in Fig. 3. | S28 |
| S22 | Light-sheet intensity profiles for the data shown in Fig. 4. | S30 |

| **Table #** | **Description** | **Page #** |
|---|---|---|
| S3 | Experimental parameters for all data shown in Main Text. | S31 |

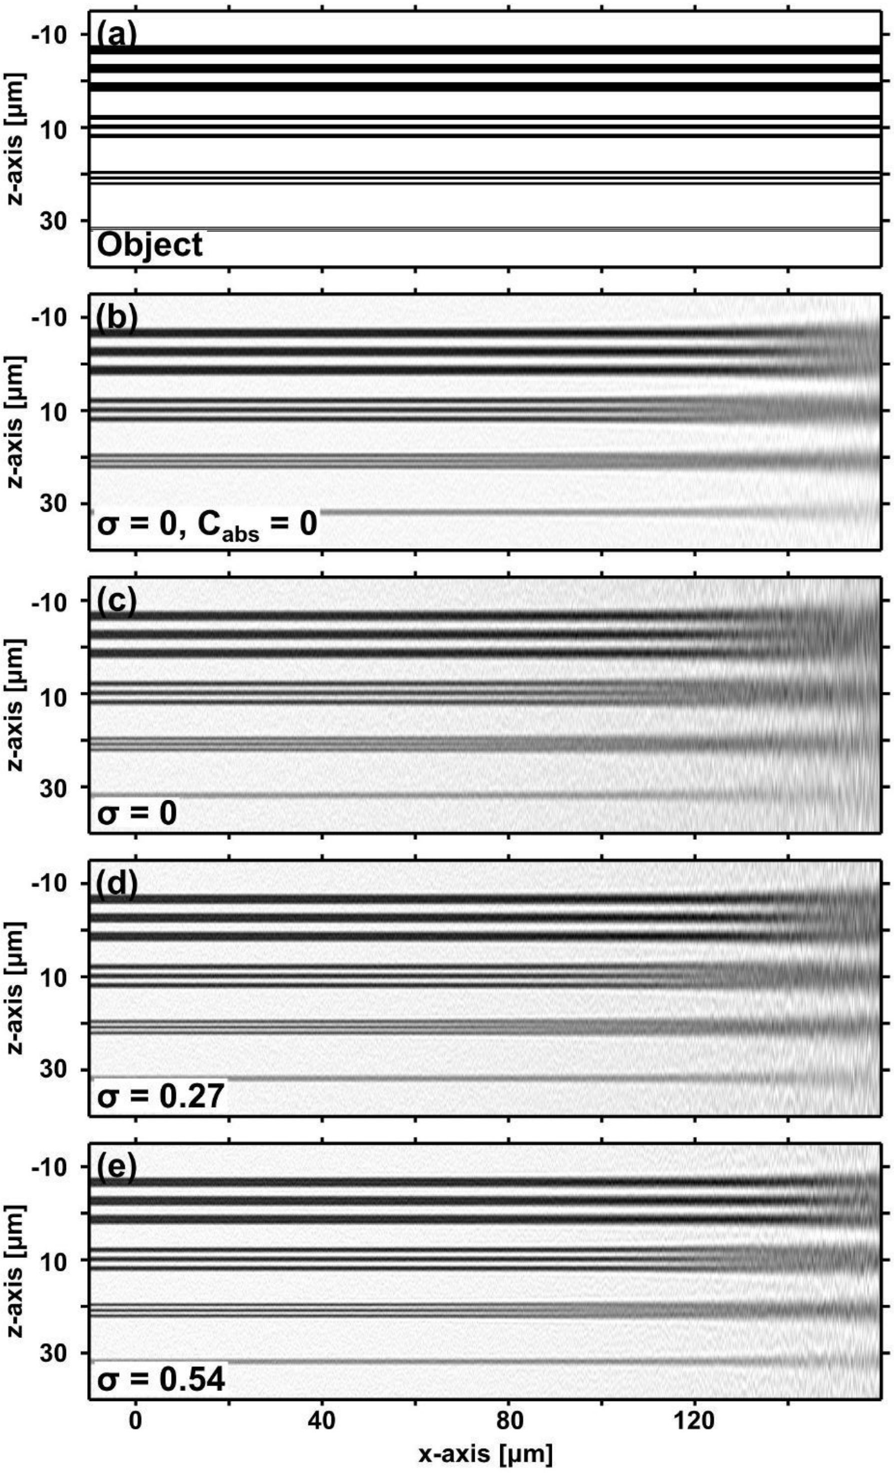


Figure S18: Simulated images of a 1D resolution target shown in (a). Simulated deconvolved Airy LSM images (b-e), in a sample with no absorption (attenuation) (b) and with an absorption coefficient $C_{abs} = 64.95\text{cm}^{-1}$ (c-e). $\sigma = 0.54$ completely counteracts the attenuation. Line width/spacing: 2 µm (top), 1 µm, 0.6 µm, 0.2 µm (bottom).

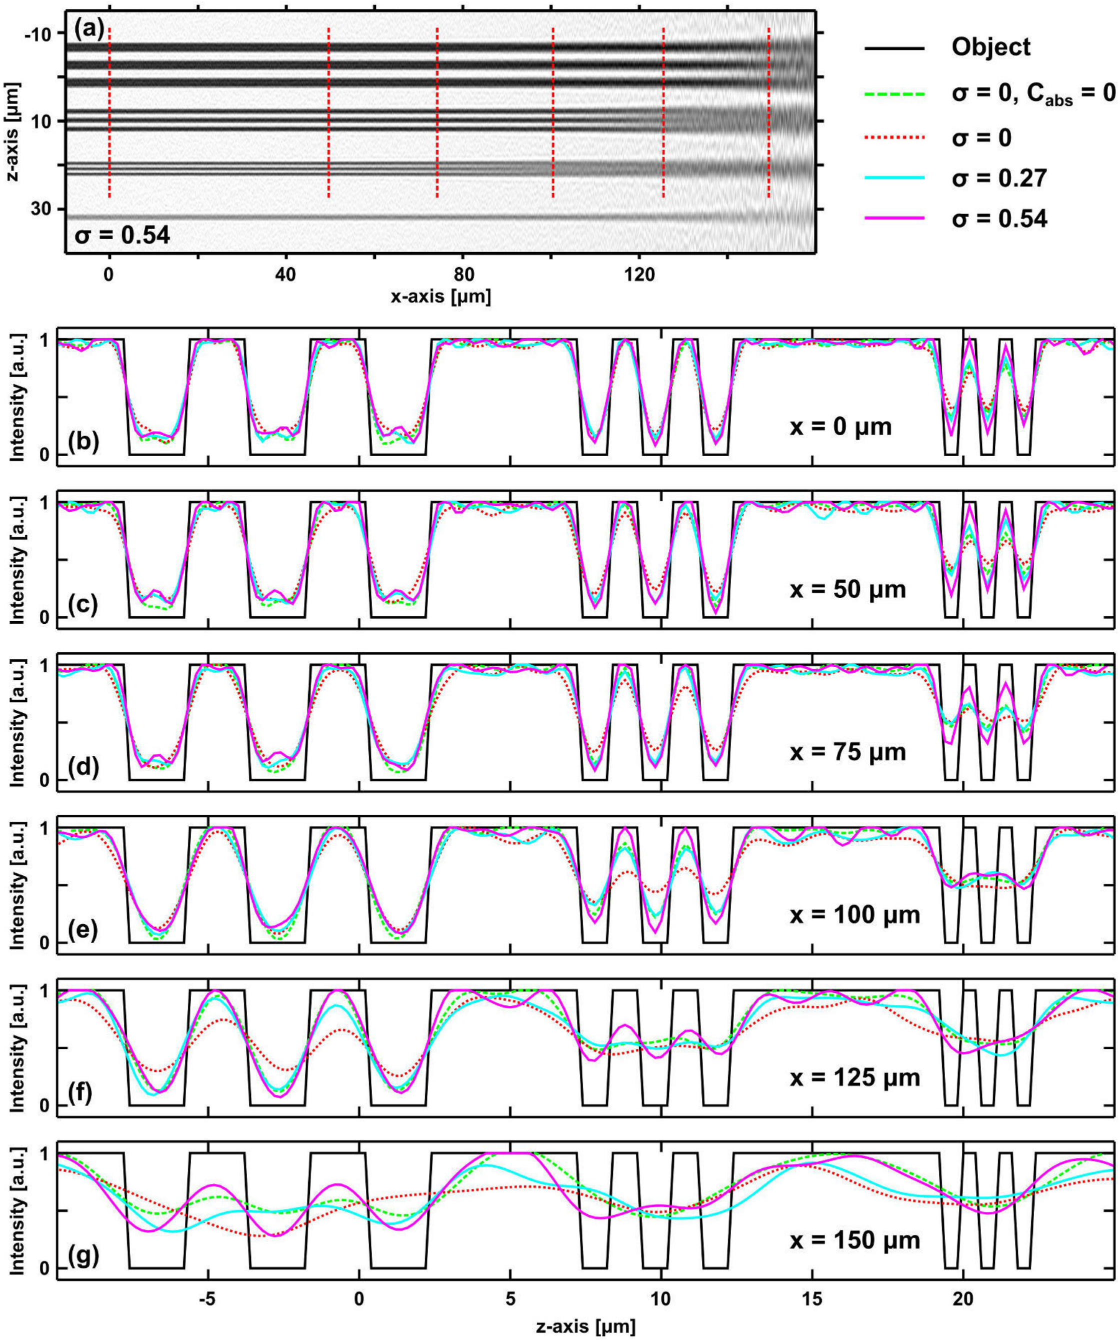


Figure S19: Intensity profiles through simulated Airy LSM images of the 1D resolution target shown in Fig. S19. Intensity profiles are taken at the locations shown in (a). (b) $x = 0\,\mu\text{m}$, (c) $x = 50\,\mu\text{m}$, (d) $x = 75\,\mu\text{m}$, (e) $x = 100\,\mu\text{m}$, (f) $x = 125\,\mu\text{m}$, (g) $x = 150\,\mu\text{m}$. Line width/spacing: $2\,\mu\text{m}$ (top), $1\,\mu\text{m}$, $0.6\,\mu\text{m}$, $0.2\,\mu\text{m}$ (bottom).

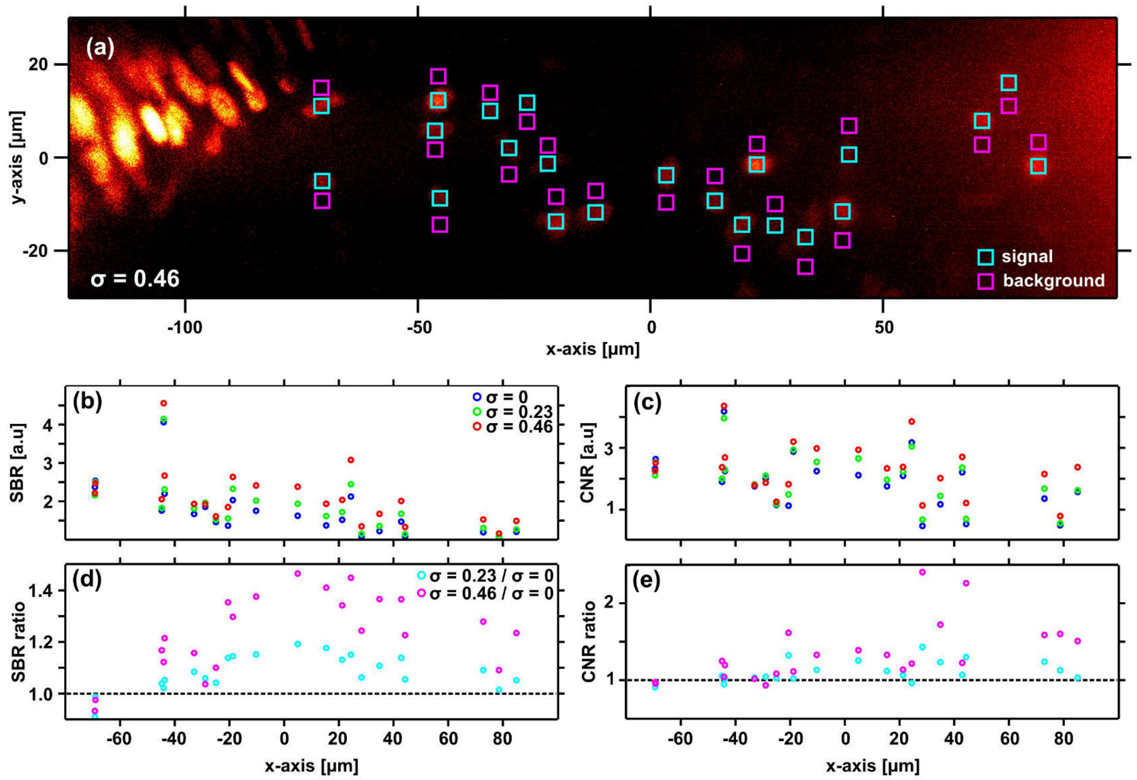


Figure S20: (a) Maximum intensity projection of deconvolved Airy LSM image of nuclei (propidium iodide) in the operculum of *S. lamarcki* (attenuation estimated at 85cm$^{-1}$) with $\sigma = 0.46$ as shown in Fig. 3. $3 \times 3\,\mu m^2$ signal regions are highlighted by cyan squares on identified nuclei. Background regions were selected in close proximity, and on the same $x-$axis coordinate, to identified nuclei as shown by magenta squares. (b,c) Local signal-to-background ratio (SBR) and contrast-to-noise ratio (CNR) plotted as a function of propagation coordinate, $x$, for $\sigma = 0$ (blue), $\sigma = 0.23$ (green), and $\sigma = 0.46$ (red). (d,e) Ratios of SBR and CNR with $\sigma = 0.23$ (cyan) and $\sigma = 0.46$ (magenta) to $\sigma = 0$. Even with partial attenuation-compensation, an improvement in the SBR and CNR is observed. With $\sigma = 0.23$, the effective attenuation after compensation is $C'_{attn} = 57.5\text{cm}^{-1}$ and an improvement of between $5-20\%$ in SBR and $5-50\%$ in CNR is observed. With $\sigma = 0.46$, the effective attenuation after compensation is $C'_{attn} = 30\text{cm}^{-1}$ and an improvement of between $20-45\%$ in SBR and $20-140\%$ in CNR is observed.

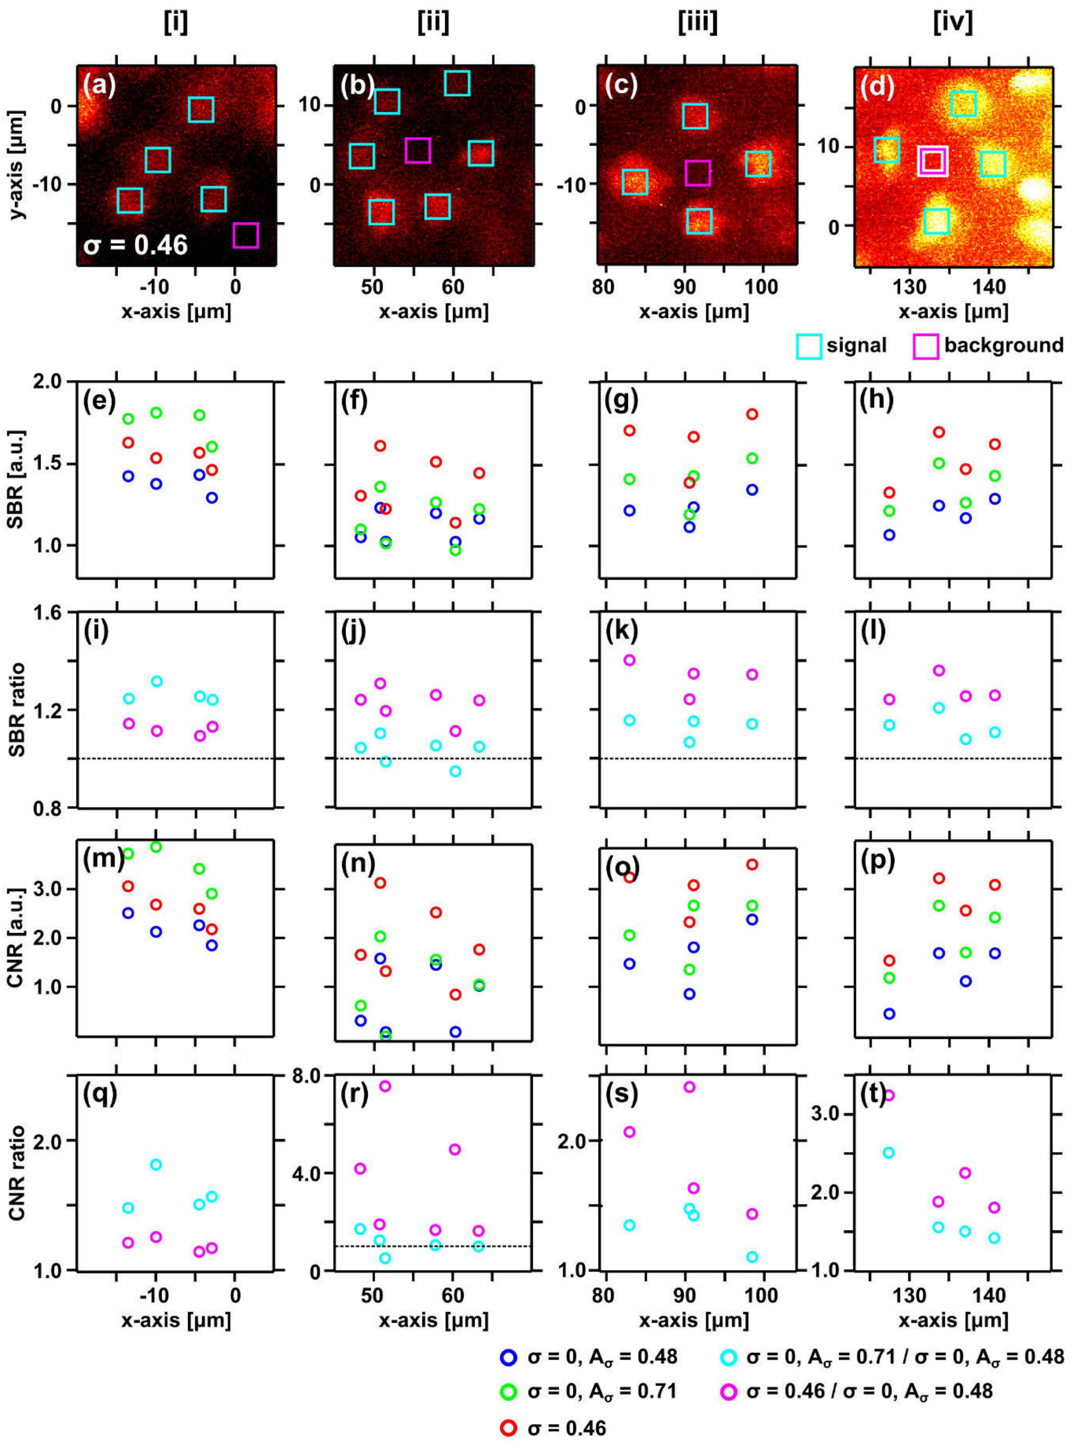


Figure S21: (a-d) Maximum intensity projection of deconvolved Airy LSM image of nuclei (propidium iodide) in the operculum of *S. lamarcki* (attenuation estimated at $75\text{cm}^{-1}$) with $\sigma = 0.46$ as shown in Fig. 4. Regions [i]-[iv] indicate the same regions highlighted in Fig. 4. $3 \times 3\,\mu\text{m}^2$ signal regions are highlighted by cyan squares on identified nuclei. Background regions were selected in close proximity to identified nuclei as shown by magenta squares. The same background region was used for all signal regions within the ROI. (e-h) Local signal-to-background ratio (SBR) plotted as a function of propagation coordinate, $x$, for $\sigma = 0$, $A_\sigma = 0.48$ (blue), $\sigma = 0$, $A_\sigma = 0.71$ (green), and $\sigma = 0.46$ (red). (i-l) Ratios of SBR with $\sigma = 0$, $A_\sigma = 0.71$ (cyan) and $\sigma = 0.46$ (magenta) to (continued on next page)

Figure S21: (continued from previous page) $\sigma = 0$, $A_\sigma = 0.48$. In regions [ii]-[iv], the use of compensation (red/magenta) increases the SBR by $20-40\%$ whereas increasing the power without attenuation-compensation (green/cyan) increased the SBR by only $0-20\%$. In region [i], increasing the power without attenuation-compensation improves the SBR more than the use of attenuation-compensation but this is expected given the significant increase in intensity in the non-compensated light-sheet at this point (see Fig. S22). (m-p) local contrast-to-noise ratio (CNR) plotted as a function of propagation coordinate for the same illumination schemes and (q-t) the ratios of CNR with $\sigma = 0$, $A_\sigma = 0.71$ (cyan) and $\sigma = 0.46$ (magenta) to $\sigma = 0$. At $x \approx 60\,\mu\text{m}$ a datapoint for the case of $\sigma = 0$, $A_\sigma = 0.71$ (green.cyan) is missing from (n,r). The CNR for this feature was negative, owing to low signal, and therefore the CNR ratio relative to the case of $\sigma = 0$, $A_\sigma = 0.48$ is ill defined. The same trend is observed for CNR as for SBR. In regions [ii]-[iv] the use of compensation increased the CNR by $50 - 650\%$.

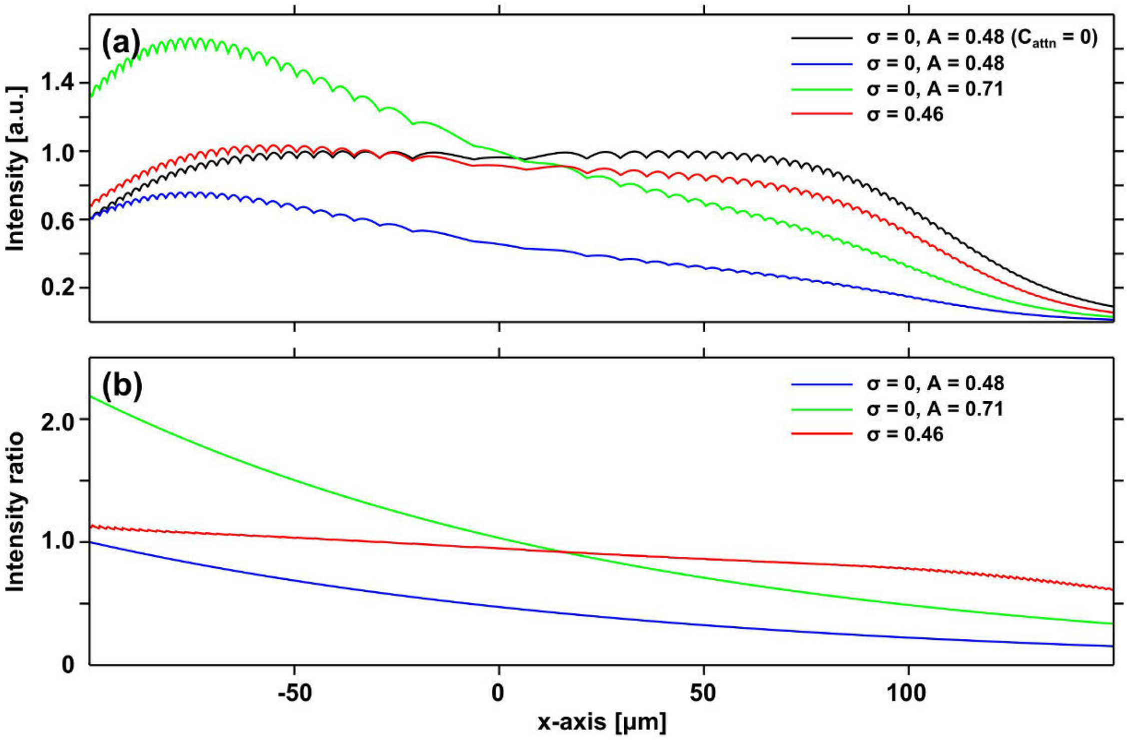


Figure S22: (a) The integrated intensity profiles of simulated Airy light-sheets as a function of propagation distance as used for deconvolution in Fig. 4. Black: uncompensated, unattenuated (ideal) light-sheet ($\sigma = 0$, $C_{attn} = 0$). Blue: uncompensated light-sheet with $C_{attn} = 75\text{cm}^{-1}$ applied. Red: compensated light-sheet with $\sigma = 0.46$ and $C_{attn} = 75\text{cm}^{-1}$. Green: an uncompensated light-sheet with $C_{attn} = 0$ and $\sigma = 0$, and the amplitude factor increased to $A_\sigma = 0.71$ such that its total power is equal to that of the compensated light-sheet (red). (b) Ratios of the attenuated and/or compensated light-sheet profiles to the ideal light-sheet (black curve in (a)). Blue: the attenuated, uncompensated light-sheet decays exponentially with propagation distance. Green: the peak power delivered by the attenuated, high-power light-sheet is more than twice the power delivered by the ideal light-sheet. However, it also decays exponentially into the medium. Red: due to strategic redistribution of power, the peak power delivered by the compensated light-sheet is never more than 10% greater than the power of the original, even though its power at the back aperture is equal to that of the high-powered beam (green). Its intensity profile is much flatter, and it stays within 10% of the intensity of the ideal beam over a distance of about 150 µm.

| Fig # | Sample | System type | Light-sheet parameters | | | Illumination power | | | Acquisition parameters | | $C^D_{attn}$ [cm$^{-1}$] |
|---|---|---|---|---|---|---|---|---|---|---|---|
| | | | $\alpha$ | $\sigma$ | $A_\sigma$ | $P^{Th}_{rel}$ | $P^{Exp}_{rel}$ | $P$ [µW] | $t_{int}$ [ms] | $z-$spacing [µm] | |
| 2 | Absorbing phantom | DLSM | 7 | 0 | 0.48 | 1 | 1 | $140 \pm 5$ | 25 | 0.2 | 55 |
| | | | | 0.23 | 0.70 | 1.38 | $1.37 \pm 0.04$ | $190 \pm 5$ | | | |
| | | | | 0.46 | 1.07 | 2.21 | $2.26 \pm 0.04$ | $315 \pm 5$ | | | |
| 3 | *S. lamarki* | DLSM | 7 | 0 | 0.48 | 1 | 1 | $140 \pm 5$ | 50 | 0.4 | 85 |
| | | | | 0.23 | 0.70 | 1.38 | $1.37 \pm 0.04$ | $190 \pm 5$ | | | |
| | | | | 0.46 | 1.07 | 2.21 | $2.26 \pm 0.04$ | $315 \pm 5$ | | | |
| 4 | *S. lamarki* | DLSM | 7 | 0 | 0.48 | 1 | 1 | $140 \pm 5$ | 50 | 0.4 | 75 |
| | | | | 0 | 0.71 | 2.19 | $2.14 \pm 0.04$ | $300 \pm 5$ | | | |
| | | | | 0.46 | 1.07 | 2.21 | $2.26 \pm 0.04$ | $315 \pm 5$ | | | |
| 5 | Mouse brain section | SPIM | 7 | 0 | 0.48 | 1 | 1 | $1420 \pm 10$ | 100 | 0.2 | 100 |
| | | | | 0.54 | 1.23 | 2.59 | $2.57 \pm 0.02$ | $3650 \pm 10$ | | | |

Table S3: Experimental parameters for all data shown in Main Text. $P^{Th}_{rel}$: Relative power (with respect to a non-compensated Airy light-sheet ($\alpha = 7$, $\sigma = 0$, $A_\sigma = 0.48$)) determined by theory, $P^{Exp}_{rel}$: relative power determined experimentally, $P$: absolute experimental power, $t_{int}$: camera integration time, $c^D_{attn}$: estimated attenuation coefficient used in deconvolution procedure.

## References


[1] J. Huisken, J. Swoger, F. Del Bene, J. Wittbrodt, and E. H. K. Stelzer, "Optical sectioning deep inside live embryos by selective plane illumination microscopy," Science **305**(5686), 1007-1009 (2004).

[2] B. Höckendorf, T. Thumberger, and J. Wittbrodt, "Quantitative Analysis of Embryogenesis: A Perspective for Light Sheet Microscopy," Developmental Cell **23**,(6), 1111-1120 (2012).

[3] M. B. Ahrens, M. B. Orger, D. N. Robson, J. M. Li, and P. J. Keller, "Whole-brain functional imaging at cellular resolution using light-sheet microscopy," Nature Methods **10**, 413-420 (2013).

[4] Z. Yang, P. Haslehurst, S. Scott, N. Emptage, and K. Dholakia, "A compact light-sheet microscope for the study of the mammalian central nervous system," Scientific Reports **6**, 26317 (2016).

[5] N. Ji, "Adaptive optical fluorescence microscopy," Nature Methods **14**, 374-380 (2017).

[6] R. M. Power and J. Huisken, "A guide to light-sheet fluorescence microscopy for multiscale imaging," Nature Methods **14**, 360-373 (2017).

[7] H. I. C. Dalgarno, T. Čižmár, T. Vettenburg, J. Nylk, F. J. Gunn-Moore, and K. Dholakia, "Wavefront corrected light sheet microscopy in turbid media," Applied Physics Letters **100**, 191108 (2012).

[8] C. Bourgenot, C. D. Saunter, J. M. Taylor, J. M. Girkin, and G. D. Love, "3D adaptive optics in a light sheet microscope," Optics Express **20**(12), 13252-13261 (2012).

[9] A. Masson, P. Escande, C. Frongia, G. Clouvel, B. Ducommun, and C. Lorenzo, "High-resolution in-depth imaging of optically cleared thick samples using an adaptive SPIM," Scientific Reports **5**, 16898 (2015).

[10] D. Wilding, P. Pozzi, O. Soloviev, G. Vdovin, and M. Verhaegen, "Adaptive illumination based on direct wavefront sensing in a light-sheet fluorescence microscope," Optics Express **24**(22), 24896-24906 (2016).

[11] T. Vettenburg, H. I. C. Dalgarno, J. Nylk, C. Coll-Lladó, D. E. K. Ferrier, T. Čižmár, F. J. Gunn-Moore, and K. Dholakia, "Light-sheet microscopy using an Airy beam," Nature Methods **11**, 541-544 (2014).

[12] Z. Yang, M. Prokopas, J. Nylk, C. Coll-Lladó, F. J. Gunn-Moore, D. E. K. Ferrier, and K. Dholakia, "A compact Airy beam light sheet microscope with a tilted cylindrical lens," Biomedical Optics Express **5**(10), 3434-3442 (2014).

[13] P. Piksarv, D. Marti, T. Le, A. Unterhuber, L. H. Forbes, M. R. Andrews, A. Stingl, W. Drexler, P. E. Andersen, and K. Dholakia, "Integrated single- and two-photon light sheet microscopy using accelerating beams," Scientific Reports **7**, 1435 (2017).

[14] F. O. Fahrbach and A. Rohrbach, "A line scanned light-sheet microscope with phase shaped self-reconstructing beams," Optics Express **18**(23), 24229-24244 (2010).

[15] O. E. Olarte, J. Licea-Rodriguez, J. A. Palero, E. J. Gualda, D. Artigas, J. Mayer, J. Swoger, J. Sharp, I. Rocha-Mendoza, R. Rangel-Rojo, and P. Loza-Alvarez, "Image formation by linear and nonlinear digital scanned light-sheet fluorescence microscopy with Gaussian and Bessel beam profiles," Biomedical Optics Express **3**(7), 1492-1505 (2012).

[16] T. A. Planchon, L. Gao, D. E. Milkie, M. W. Davidson, J. A. Galbraith, C. G. Galbraith, and E. Betzig, "Rapid three-dimensional isotropic imaging of living cells using Bessel beam plane illumination," Nature Methods **8**, 417-423 (2011).

[17] L. Gao, L. Shao, C. D. Higgins, J. S. Poulton, M. Peifer, M. W. Davidson, X. Wu, B. Goldstein, and E. Betzig, "Noninvasive imaging beyond the diffraction limit of 3D dynamics in thickly fluorescent specimens," Cell **151**(6), 1370-1385 (2012).

[18] B.-C. Chen, W. R. Legant, K. Wang, L. Shao, D. E. Milkie, M. W. Davidson, C. Janetopoulos, X. S. Wu, J. A. Hammer III, Z. Liu, B. P. English, Y. Mimori-Kiyosue, D. P. Romero, A. T. Ritter, J. Lippincott-Schwartz, L. Fritz-Laylin, R. D. Mullins, D. M. Mitchell, J. N. Bembenek, A.-C. Reymann, R. Böhme, S. W. Grill, J. T. Wang, G. Seydoux, U. S. Tulu, D. P. Kiehart, and E. Betzig, "Lattice light-sheet microscopy: imaging molecules to embryos at high spatiotemporal resolution," Science **346**(6208), 1257998 (2014).

[19] Z. Bouchal, J. Wagner, and M. Chlup, "Self-reconstruction of a distorted nondiffracting beam," Optics Communications **151**(4-6), 207-211 (1998).

[20] J. Broky, G. A. Siviloglou, A. Dogariu, and D. N. Christodoulides, "Self-healing properties of optical Airy beams," Optics Express **16**(17), 12880-12891 (2008).

[21] M. Mazilu, D. J. Stevenson, F. Gunn-Moore, and K. Dholakia, "Light beats the spread: "non-diffracting" beams," Laser Photonics Review **4**(4), 529-547 (2010).

[22] X. Chu, G. Zhou, and R. Chen, "Analytical study of the self-healing property of Airy beams," Physical Review A **85**, 013815 (2012).

[23] L. Zhang, F. Ye, M. Cao, D. Wei, P. Zhang, H. Gao, and F. Li, "Investigating the self-healing property of an optical Airy beam," Optics Letters **40**(21), 5066-5069 (2015).

[24] F. O. Farhbach and A. Rohrbach, "Propagation stability of self-reconstructing Bessel beams enables contrast-enhanced imaging in thick media," Nature Communications **3**, 1646 (2012).

[25] Y. Chen and J. T. C. Liu, "Characterizing the beam steering and distortion of Gaussian and Bessel beams focused in tissues with microscopic heterogeneities," Biomedical Optics Express **6**(4), 1318-1330 (2015).

[26] J. Nylk, K. McCluskey, S. Aggarwal, J. A. Tello, and K. Dholakia, "Enhancement of image quality and imaging depth with Airy light-sheet microscopy in cleared and non-cleared neural tissue," Biomedical Optics Express **7**,(10), 4021-4033 (2016).

[27] T. Čižmár and K. Dholakia, "Tunable Bessel light modes: engineering the axial propagation," Optics Express **17**(18), 15558-15570 (2009).

[28] M Zamboni-Rached, "Stationary optical wave fields with arbitrary longitudinal shape by superposing equal frequency Bessel beams: Frozen Waves," Optics Express **12**(17), 4001-4006 (2004).

[29] M. A. Preciado and K. Sugden, "Proposal and design of Airy-based rocket pulses for invariant propagation in lossy dispersive media," Optics Letters **37**(23), 4970-4972 (2012).

[30] M. A. Preciado, K. Dholakia, and M. Mazilu, "Generation of attenuation-compensating Airy beams," Optics Letters **39**(16), 4950-4953 (2014).

[31] R. Schley, I. Kaminer, E. Greenfield, R. Bekenstein, Y. Lumer, and M. Segev, "Loss-proof self-accelerating beams and their use in non-paraxial manipulation of particles' trajectories," Nature Communications **5**, 5189 (2014).

[32] J. Nylk, K. McCluskey, M. A. Preciado, M. Mazilu, F. J. Gunn-Moore, S. Aggarwal, J. A. Tello, D. E. K. Ferrier, and K. Dholakia, "Data underpinning: Light-sheet microscopy with attenuation-compensated propagation-invariant beams," http://dx.doi.org/10.17630/b5ebd26e-dd89-45ca-8478-e9d2f08e5975

[33] P. Zhang, M. E. Phipps, P. M. Goodwin, and J. H. Werner, "Confocal line scanning of a Bessel beam for fast 3D imaging," Optics Letters **39**(12), 3682-3685 (2014).

[34] P. Zhang, M. E. Phipps, P. M. Goodwin, and J. H. Werner, "Light-sheet microscopy by confocal line scanning of dual-Bessel beams," Journal of Biomedical Optics **21**(10), 100502 (2016).

[35] R. Szabó and D. E. K. Ferrier, "Cell proliferation dynamics in regeneration of the operculum head appendage in the annelid *Pomatoceros lamarckii*," Journal of Experimental Zoology B: Molecular and Developmental Evolution **322**, 257-268 (2014).

[36] A. K. Topaloglu, J. A. Tello, L. D. Kotan, M. N. Ozbek, M. B. Yilmaz, S. Erdogan, F. Gurbuz, F. Temiz, R. P. Millar, and B. Yuskel, "Inactivating *Kiss1* Mutation and Hypgonadatropic Hypogonadism," New England Journal of Medicine **366**(7), 629-635 (2012).

[37] S. B. Seminara, S. Messager, E. E. Chatzidaki, R. R. Thresher, J. S. Acierno, J. K. Shagoury, Y. Bo-Abbas, W. Kuohung, K. M. Schwinof, A. G. Hendrick, D. Zahn, J. Dixon, U. B. Kaiser, S. A. Slaugenhaupt, J. F. Gusella, S. O'Rahilly, M. B. L. Carlton, W. F. Crowley, S. A. J. R. Aparicio, and W. H. Colledge, "The *GPR54* Gene as a Regulator of Puberty," New England Journal of Medicine **349**(17), 1614-1627 (2003).

[38] M. Cholanian, S. J. Krajewski-Hall, N. T. McMullen, and N. E. Rance, "Chronic Oestradiol Reduces the Dendritic Spine Density of KNDy (Kisspeptin/Neurokinin B/Dynorphin) Neurones in the Arcuate Nucleus of Ovariectomised Tac2-Enhanced Green Gluorescent Protein Transgenic Mice," J. Neuroendocrinology **27**(4), 253-263 (2015).

[39] P. J. Keller, A. D. Schmidt, J. Wittbrodt, and E. H. K. Stelzer, "Reconstruction of zebrafish early embryonic development by scanned light sheet microscopy," Science **322**(5904), 1065-1069 (2008).

[40] M. Jemielita, M. J. Taormina, A. DeLaurier, C. B. Kimmel, and R. Parthasarathy, "Comparing phototoxicity during the development of a zebrafish craniofacial bone using confocal and light sheet fluorescence microscopy techniques," Journal of Biophotonics **6**(11-12), 920-928 (2013).

[41] P. P. Laissue, R. A. Alghamdi, P. Tomancak, E. G. Raynaud, and H. Shroff, "Assessing phototoxicity in live fluorescence imaging," Nature Methods **14**, 657-661 (2017).

[42] J. Swoger, P. Verveer, K. Greger, J. Huisken, and E. H. K. Stelzer, "Multi-view image fusion improves resolution in three-dimensional microscopy," Optics Express **15**(13), 8029-8042 (2007).

[43] U. Krzic, S. Gunther, T. E. Saunders, S. J. Streichan, and L. Hufnagel, "Multiview light-sheet microscope for rapid *in toto* imaging," Nature Methods **9**, 730-733 (2012).

[44] G. de Medeiros, N. Norlin, S. Gunther, M. Albert, L. Panavaite, U.-M. Fiuza, F. Peri, T. Hiiragi, U. Krzic, and L. Hufnagel, "Confocal multiview light-sheet microscopy," Nature Communications **6**, 8881 (2015).

[45] Y. Wu, P. Chandris, P. W. Winter, E. Y. Kim, V. Jaumouillé, A. Kumar, M. Guo, J. M. Leung, C. Smith, I. Rey-Suarez, H. Liu, C.M. Waterman, K. S. Ramamurthi, P. J. La Riviere, and H. Shroff, "Simultaneous multiview capture and fusion improves spatial resolution in wide-field and light-sheet microscopy," Optica **3**(8), 897-910 (2016).

[46] D. C. Adler, T. H. Ko, and J. G. Fujimoto, "Speckle reduction in optical coherence tomography images by use of a spatially adaptive wavelet filter," Optics Letters **29**(24), 2878-2880 (2004).

[47] C. McClure, K. L. H. Cole, P. Wulff, M. Klugmann, and A. J. Murray, "Production and Titering of Recombinant Adeno-associated Viral Vectors," Journal of Visualized Experiments **57**, e3348 (2011).
